# Supplementary material for: Automation and Taxation
Source: arXiv:2103.04111 source file (2022-04-21)
Supplement: Supplementary file 1 [file Sumstat_controls_ct_SI.tex]

\multicolumn{20}{l}{SI} \\\midrule
Mean        &          37&          15&           8&          14&          41&          22&          37&          21&         7.6&          62&         2.2&          51&         .15&          42&           2&        -3.9&         4.2&         .12&         .56\\
St.Dev.     &         .55&         .53&          .7&         .57&         1.1&         1.7&         1.9&         4.1&         1.7&          13&         3.4&         2.1&       .0098&          22&         .67&         3.4&         .57&       .0078&        .014\\
Min         &          36&          14&         6.9&          13&          39&          19&          35&          12&         4.1&          36&        -7.5&          49&         .13&          22&         1.1&         -15&         3.1&         .11&         .55\\
Median      &          37&          15&         7.9&          14&          40&          21&          37&          23&           8&          69&         3.2&          50&         .14&          27&         1.9&        -2.8&         4.1&         .12&         .56\\
Max         &          38&          16&         9.2&          15&          43&          25&          40&          25&         9.5&          76&           7&          54&         .16&          83&         3.2&           0&         5.1&         .14&         .58\\\bottomrule
