# Supplementary material for: Automation and Taxation
Source: arXiv:2103.04111 source file (2022-04-21)
Supplement: Supplementary file 3 [file suppl_material.tex]

\appendix

 \setcounter{section}{0}
 \setcounter{figure}{0}
 \setcounter{table}{0}
 \setcounter{equation}{0}
%\part*{SUPPLEMENTARY MATERIAL --- ONLINE APPENDIX}
\section{Additional regression results}
\subsection{Prerequisites}
\subsubsection{Further determinants of taxation}
\label{appendix:add_results_determinants_taxation}
    Here, we briefly outline other determinants of taxation that are included in the regressions but not discussed in the main text. These regressors are motivated by the literature and taxation and cover GDP growth, the market share of services $Services_{c,t}$, public finance related indicators (debt, interest payments and deficit), measures for industrial concentration $HHI_{c,t}$, the exchange rate $XRate_{c,t}$ (i.e. US\$ per Euro) as proxy for trade and public investments $GovInvest^{\%GDP}_{c,t}$. 
    
	Labor taxes in absolute terms, in relation to GDP and as share in total taxation exhibit a positive correlation with the service share. 
	This pattern holds for the majority of sub-periods and regions. In other sub-samples, we additionally find a negative association of the services share with taxes on capital and goods. Northern Europe is an exception where we observe a weakly significant opposite relationship. 	

    High indebtedness and higher deficits are positively related to taxes in absolute terms and measured in percentage GDP. 
    %This relationship is reversed in some regions after the financial crisis 2008. 
    Net lending as percentage GDP is positively correlated with all taxes except from labor taxes which are negatively related to deficits. 
    
	We find a higher exchange rate $XRate_{c,t}$ to be negatively related to taxes on capital, goods and in total measured in absolute terms and as percentage of GDP. We also observe a higher exchange rate to be positively related to the relative tax contribution of labor at the cost of taxes on capital. This relationship is opposite in Southern European countries.\footnote{Note that the exchange rate varies across European countries only in the time dimension since the EU's Exchange Rate Mechanism aims to keep exchange rate fluctuations between the Euro and other European currencies flat (see also \url{https://stats.oecd.org/glossary/detail.asp?ID=3055}). Hence, $XRate_{c,t}$ captures the competitiveness of European countries on global markets but can not be interpreted as an indicator for within-European trade.}

	\begin{table}[H]
	{\centering 
     
    \caption{Taxation and the structure of production}
    
    \label{tab:regr_pre_tax_prod6}
    \begin{adjustbox}{width=\textwidth}\begin{tabular}{l|cccc|cccc|ccc}
    \toprule \addlinespace
\csname @@input\endcsname{inputs/all_95_16/Results2RICTint_ct_All_95t16}
\bottomrule
    \end{tabular}\end{adjustbox} \\ } \scriptsize
   Notes: \sym{*}\(p<0.05\), \sym{**}\(p<0.01\), \sym{***}\(p<0.001\). Regression results to examine the link between tax aggregation and economic production for 19 European countries during the period 1995-2016. All regressions use country level data and include: GDP growth ($GDPgrowth_{c,t}$); share of gross output produced in service industries ($Services_{c,t}$); Herfindahl-Hirschman Index based on the gross output shares of macro-sectors ($HHI_{c,t}$); government consolidated gross debt as \% of GDP ($Debt^{\%GDP}_{c,t}$); government interest payable as \% of GDP ($Interest^{\%GDP}_{c,t}$); net government lending/borrowing as \% of GDP ($Lending^{\%GDP}_{c,t}$); gross fixed capital formation as \% of GDP ($GovInv^{\%GDP}_{c,t}$); period average exchange rate ($XRate_{c,t}$); and country ($c$) and year ($t$) fixed effects. For the first block (Taxes in ln of national currency), $wL_{c,t}$, $rK_{c,t}$ and $pQ_{c,t}$ are expressed as the natural logarithm ($ln$) while for the last two blocks they are expressed as \% of GDP. Standard errors are clustered both at the country and year level.
    \end{table}
\newpage

	\begin{table}[!hb]
	{\centering 
     
    \caption{Taxation and the structure of production before 2007 in whole Europe}
    \begin{adjustbox}{width=\textwidth}\begin{tabular}{l|cccc|cccc|ccc}
    \toprule \addlinespace
\csname @@input\endcsname{inputs/all_subperiod/Results2RICTint_ct_All_95t07}
\bottomrule
    \end{tabular}\end{adjustbox} \\ }
        \scriptsize
   Notes: \sym{*}\(p<0.05\), \sym{**}\(p<0.01\), \sym{***}\(p<0.001\). Regression results to examine the link between tax aggregation and economic production  for 19 European countries during the period 1995-2007. All regressions use country level data and include: GDP growth ($GDPgrowth_{c,t}$); share of gross output produced in service industries ($Services_{c,t}$); Herfindahl-Hirschman Index based on the gross output shares of macro-sectors ($HHI_{c,t}$); government consolidated gross debt as \% of GDP ($Debt^{\%GDP}_{c,t}$); government interest payable as \% of GDP ($Interest^{\%GDP}_{c,t}$); net government lending/borrowing as \% of GDP ($Lending^{\%GDP}_{c,t}$); gross fixed capital formation as \% of GDP ($GovInv^{\%GDP}_{c,t}$); period average exchange rate ($XRate_{c,t}$); and country ($c$) and year ($t$) fixed effects. For the first block, $wL_{c,t}$, $rK_{c,t}$ and $pQ_{c,t}$ are expressed as the natural logarithm ($ln$) while for the last two blocks they are expressed as \% of GDP.
    \end{table}
\newpage
	\begin{table}[H]
	{\centering 
     
    \caption{Taxation and the structure of production after 2008 in whole Europe}
    \begin{adjustbox}{width=\textwidth}\begin{tabular}{l|cccc|cccc|ccc}

    \toprule \addlinespace
\csname @@input\endcsname{inputs/all_subperiod/Results2RICTint_ct_All_08t16}
\bottomrule
    \end{tabular}\end{adjustbox} \\ }
    %%\label{tab:regr_pre_tax_prod6}
        \scriptsize
   Notes: \sym{*}\(p<0.05\), \sym{**}\(p<0.01\), \sym{***}\(p<0.001\). Regression results to examine the link between tax aggregation and economic production for 19 European countries during the period 2008-2016. All regressions use country level data and include: GDP growth ($GDPgrowth_{c,t}$); share of gross output produced in service industries ($Services_{c,t}$); Herfindahl-Hirschman Index based on the gross output shares of macro-sectors ($HHI_{c,t}$); government consolidated gross debt as \% of GDP ($Debt^{\%GDP}_{c,t}$); government interest payable as \% of GDP ($Interest^{\%GDP}_{c,t}$); net government lending/borrowing as \% of GDP ($Lending^{\%GDP}_{c,t}$); gross fixed capital formation as \% of GDP ($GovInv^{\%GDP}_{c,t}$); period average exchange rate ($XRate_{c,t}$); and country ($c$) and year ($t$) fixed effects. For the first block, $wL_{c,t}$, $rK_{c,t}$ and $pQ_{c,t}$ are expressed as the natural logarithm ($ln$) while for the last two blocks they are expressed as \% of GDP.
    \end{table}

\FloatBarrier
\subsubsection{Taxation and automation by region and period}
\label{appendix:add_results_taxes_and_ai}
    \begin{table}[H]
    \caption{Taxation and automation in Eastern Europe}
    {\centering
    \begin{adjustbox}{width=\textwidth}\begin{tabular}{l|cccc|cccc|ccc}
    \toprule \addlinespace
\csname @@input\endcsname{inputs/east_95_16/Results2shortV1_RICTint_ct_East_95t16}
\midrule
\csname @@input\endcsname{inputs/east_subperiod/Results2shortV1_RICTint_ct_East_95t07}
\midrule
\csname @@input\endcsname{inputs/east_subperiod/Results2shortV1_RICTint_ct_East_08t16}
\bottomrule
    \end{tabular}\end{adjustbox}} \\ 
    \label{tab:regr_pre_tax_robots_east} \scriptsize
  Notes: \sym{*}\(p<0.05\), \sym{**}\(p<0.01\), \sym{***}\(p<0.001\). Regression results of aggregate flows of tax revenues on different automation measures for Eastern European countries during the period 1995-2016. All regressions use country level data and include: GDP growth, gross output share of service industries; Herfindahl-Hirschman Index based on the gross output shares of macro-sectors; government consolidated gross debt as \% of GDP; government interest payable as \% of GDP; net government lending/borrowing as \% of GDP; gross fixed capital formation as \% of GDP; period average exchange rate; and country ($c$) and year ($t$) fixed effects. All regressions for Taxes in ln of national currency also include the ln of gross output value ($pQ$). Standard errors are clustered both at the country and year level.
    \end{table}
    
    \begin{table}[H]
    \caption{Taxation and automation in Northern Europe}
    {\centering
    \begin{adjustbox}{width=\textwidth}\begin{tabular}{l|cccc|cccc|ccc}
    \toprule \addlinespace
\csname @@input\endcsname{inputs/north_95_16/Results2shortV1_RICTint_ct_North_95t16}
\midrule
\csname @@input\endcsname{inputs/north_subperiod/Results2shortV1_RICTint_ct_North_95t07}
\midrule
\csname @@input\endcsname{inputs/north_subperiod/Results2shortV1_RICTint_ct_North_08t16}
\bottomrule
    \end{tabular}\end{adjustbox}} \\ 
    \label{tab:regr_pre_tax_robots_north} \scriptsize
  Notes: \sym{*}\(p<0.05\), \sym{**}\(p<0.01\), \sym{***}\(p<0.001\). Regression results of aggregate flows of tax revenues on different automation measures for Northern European countries during the period 1995-2016. All regressions use country level data and include: GDP growth, gross output share of service industries; Herfindahl-Hirschman Index based on the gross output shares of macro-sectors; government consolidated gross debt as \% of GDP; government interest payable as \% of GDP; net government lending/borrowing as \% of GDP; gross fixed capital formation as \% of GDP; period average exchange rate; and country ($c$) and year ($t$) fixed effects. All regressions for Taxes in ln of national currency also include the ln of gross output value ($pQ$). Standard errors are clustered both at the country and year level.
    \end{table}
    
    \begin{table}[H]
    \caption{Taxation and automation in Southern Europe}
    {\centering
    \begin{adjustbox}{width=\textwidth}\begin{tabular}{l|cccc|cccc|ccc}
    \toprule \addlinespace
\csname @@input\endcsname{inputs/south_95_16/Results2shortV1_RICTint_ct_South_95t16}
\midrule
\csname @@input\endcsname{inputs/south_subperiod/Results2shortV1_RICTint_ct_South_95t07}
\midrule
\csname @@input\endcsname{inputs/south_subperiod/Results2shortV1_RICTint_ct_South_08t16}
\bottomrule
    \end{tabular}\end{adjustbox}} \\ 
    \label{tab:regr_pre_tax_robots_south} \scriptsize
  Notes: \sym{*}\(p<0.05\), \sym{**}\(p<0.01\), \sym{***}\(p<0.001\). Regression results of aggregate flows of tax revenues on different automation measures for Southern European countries during the period 1995-2016. All regressions use country level data and include: GDP growth, gross output share of service industries; Herfindahl-Hirschman Index based on the gross output shares of macro-sectors; government consolidated gross debt as \% of GDP; government interest payable as \% of GDP; net government lending/borrowing as \% of GDP; gross fixed capital formation as \% of GDP; period average exchange rate; and country ($c$) and year ($t$) fixed effects. All regressions for Taxes in ln of national currency also include the ln of gross output value ($pQ$). Standard errors are clustered both at the country and year level.
    \end{table}

\newpage
\subsubsection{Taxation, automation and the economy in different regions}
\label{appendix:add_results_taxes_and_the_economy}
To control for regional differences, we split the sample into Eastern, Northern and Southern Europe which differ by tax systems, their industrial structure and the extent to which countries were hit by the financial crisis.\footnote{Descriptive statistics and time series plots illustrating the regional peculiarities can be found in Appendix \ref{appendix:descr_stats} and \ref{appendix:key_vars_by_region}.} 

In Eastern Europe, we find that robot diffusion is negatively associated with taxes on labor and goods, but we do not observe any effects of ICT. The depth of automation is positively correlated with taxes on capital and goods and a shift from taxation of labor to capital. Until 2007, the effect of $R \ast ICT_{c,t}$ on capital taxation is opposite, i.e. negative. 

In Northern Europe, we observe a negative correlation between robot diffusion and the depth of automation and labor taxes. Until 2007, robot diffusion and automation depth exhibit a negative impact on total tax revenues and capital taxation and after 2008 on taxes on goods. 
Conversely, ICT diffusion is positively related to labor taxation at the expense of taxes on capital. 

In Southern Europe, we find robots to be negatively correlated with total tax revenues and taxes on goods measured as percentage GDP. Prior to 2007, we see a negative relationship between robots and labor taxation and after 2008 with capital taxation. 
ICTs exhibit a negative association with labor taxation and we observe an increasing share of goods taxation. 

While results for Eastern and Northern Europe align with the observations made for the full sample, the findings for Southern Europe are slightly different. We find ICT to coincide with capital accumulation and to be associated with more employment, while the effect of robots on employment and wages is negative before 2007 but positive afterwards.     
    
\FloatBarrier

	\begin{table}[H]
	{\centering 
    \caption{Taxation and the structure of production in Eastern Europe}
    \begin{adjustbox}{width=\textwidth}\begin{tabular}{l|cccc|cccc|ccc}
    \toprule \addlinespace
\csname @@input\endcsname{inputs/east_95_16/Results2RICTint_ct_East_95t16}
\bottomrule
    \end{tabular}\end{adjustbox} \\ }
    %\label{tab:regr_pre_tax_prod6}
        \scriptsize
   Notes: \sym{*}\(p<0.05\), \sym{**}\(p<0.01\), \sym{***}\(p<0.001\). Regression results to examine the link between tax aggregation and economic production for Eastern European countries during the period 1995-2016. All regressions use country level data and include: GDP growth ($GDPgrowth_{c,t}$); share of gross output produced in service industries ($Services_{c,t}$); Herfindahl-Hirschman Index based on the gross output shares of macro-sectors ($HHI_{c,t}$); government consolidated gross debt as \% of GDP ($Debt^{\%GDP}_{c,t}$); government interest payable as \% of GDP ($Interest^{\%GDP}_{c,t}$); net government lending/borrowing as \% of GDP ($Lending^{\%GDP}_{c,t}$); gross fixed capital formation as \% of GDP ($GovInv^{\%GDP}_{c,t}$); period average exchange rate ($XRate_{c,t}$); and country ($c$) and year ($t$) fixed effects. For the first block (Taxes in ln of national currency), $wL_{c,t}$, $rK_{c,t}$ and $pQ_{c,t}$ are expressed as the natural logarithm ($ln$) while for the last two blocks they are expressed as \% of GDP.
    \end{table}
%    \end{landscape}

	\begin{table}[H]
	{\centering 
     
    \caption{Taxation and the structure of production in Eastern Europe before 2007}
    \begin{adjustbox}{width=\textwidth}\begin{tabular}{l|cccc|cccc|ccc}
    %\begin{adjustbox}{width=\textwidth}\begin{tabular}{p{0.6cm}|p{.95cm}p{.95cm}p{.95cm}|p{.95cm}p{.95cm}p{.95cm}|p{.95cm}p{.95cm}p{.95cm}|p{.95cm}p{.95cm}p{.95cm}}
    \toprule \addlinespace
\csname @@input\endcsname{inputs/east_subperiod/Results2RICTint_ct_East_95t07}
\bottomrule
    \end{tabular}\end{adjustbox} \\ }
    %\label{tab:regr_pre_tax_prod6}
        \scriptsize
   Notes: \sym{*}\(p<0.05\), \sym{**}\(p<0.01\), \sym{***}\(p<0.001\). Regression results to examine the link between tax aggregation and economic production for Eastern European countries during the period 1995-2007. All regressions use country level data and include: GDP growth ($GDPgrowth_{c,t}$); share of gross output produced in service industries ($Services_{c,t}$); Herfindahl-Hirschman Index based on the gross output shares of macro-sectors ($HHI_{c,t}$); government consolidated gross debt as \% of GDP ($Debt^{\%GDP}_{c,t}$); government interest payable as \% of GDP ($Interest^{\%GDP}_{c,t}$); net government lending/borrowing as \% of GDP ($Lending^{\%GDP}_{c,t}$); gross fixed capital formation as \% of GDP ($GovInv^{\%GDP}_{c,t}$); period average exchange rate ($XRate_{c,t}$); and country ($c$) and year ($t$) fixed effects. For the first block (Taxes in ln of national currency), $wL_{c,t}$, $rK_{c,t}$ and $pQ_{c,t}$ are expressed as the natural logarithm ($ln$) while for the last two blocks they are expressed as \% of GDP.
    \end{table}
%    \end{landscape}

	\begin{table}[H]
	{\centering 
     
    \caption{Taxation and the structure of production in Eastern Europe after 2008}
    \begin{adjustbox}{width=\textwidth}\begin{tabular}{l|cccc|cccc|ccc}
    %\begin{adjustbox}{width=\textwidth}\begin{tabular}{p{0.6cm}|p{.95cm}p{.95cm}p{.95cm}|p{.95cm}p{.95cm}p{.95cm}|p{.95cm}p{.95cm}p{.95cm}|p{.95cm}p{.95cm}p{.95cm}}
    \toprule \addlinespace
\csname @@input\endcsname{inputs/east_subperiod/Results2RICTint_ct_East_08t16}
\bottomrule
    \end{tabular}\end{adjustbox} \\ }
    %%\label{tab:regr_pre_tax_prod6}
        \scriptsize
   Notes: \sym{*}\(p<0.05\), \sym{**}\(p<0.01\), \sym{***}\(p<0.001\). Regression results to examine the link between tax aggregation and economic production for Eastern European countries during the period 2008-2016. All regressions use country level data and include: GDP growth ($GDPgrowth_{c,t}$); share of gross output produced in service industries ($Services_{c,t}$); Herfindahl-Hirschman Index based on the gross output shares of macro-sectors ($HHI_{c,t}$); government consolidated gross debt as \% of GDP ($Debt^{\%GDP}_{c,t}$); government interest payable as \% of GDP ($Interest^{\%GDP}_{c,t}$); net government lending/borrowing as \% of GDP ($Lending^{\%GDP}_{c,t}$); gross fixed capital formation as \% of GDP ($GovInv^{\%GDP}_{c,t}$); period average exchange rate ($XRate_{c,t}$); and country ($c$) and year ($t$) fixed effects. For the first block (Taxes in ln of national currency), $wL_{c,t}$, $rK_{c,t}$ and $pQ_{c,t}$ are expressed as the natural logarithm ($ln$) while for the last two blocks they are expressed as \% of GDP.
    \end{table}
%    \end{landscape}

\FloatBarrier

	\begin{table}[H]
	{\centering 
     
    \caption{Taxation and the structure of production in Northern Europe}
    \begin{adjustbox}{width=\textwidth}\begin{tabular}{l|cccc|cccc|ccc}
    \toprule \addlinespace
\csname @@input\endcsname{inputs/north_95_16/Results2RICTint_ct_North_95t16}
\bottomrule
    \end{tabular}\end{adjustbox} \\ }
    %\label{tab:regr_pre_tax_prod6}
        \scriptsize
   Notes: \sym{*}\(p<0.05\), \sym{**}\(p<0.01\), \sym{***}\(p<0.001\). Regression results to examine the link between tax aggregation and economic production for Northern European countries during the period 1995-2016. All regressions use country level data and include: GDP growth ($GDPgrowth_{c,t}$); share of gross output produced in service industries ($Services_{c,t}$); Herfindahl-Hirschman Index based on the gross output shares of macro-sectors ($HHI_{c,t}$); government consolidated gross debt as \% of GDP ($Debt^{\%GDP}_{c,t}$); government interest payable as \% of GDP ($Interest^{\%GDP}_{c,t}$); net government lending/borrowing as \% of GDP ($Lending^{\%GDP}_{c,t}$); gross fixed capital formation as \% of GDP ($GovInv^{\%GDP}_{c,t}$); period average exchange rate ($XRate_{c,t}$); and country ($c$) and year ($t$) fixed effects. For the first block (Taxes in ln of national currency), $wL_{c,t}$, $rK_{c,t}$ and $pQ_{c,t}$ are expressed as the natural logarithm ($ln$) while for the last two blocks they are expressed as \% of GDP.
    \end{table}
%    \end{landscape}

	\begin{table}[H]
	{\centering 
     
    \caption{Taxation and the structure of production in Northern Europe before 2007}
    \begin{adjustbox}{width=\textwidth}\begin{tabular}{l|cccc|cccc|ccc}
    %\begin{adjustbox}{width=\textwidth}\begin{tabular}{p{0.6cm}|p{.95cm}p{.95cm}p{.95cm}|p{.95cm}p{.95cm}p{.95cm}|p{.95cm}p{.95cm}p{.95cm}|p{.95cm}p{.95cm}p{.95cm}}
    \toprule \addlinespace
%\csname @@input\endcsname{inputs/north_subperiod/Results2_ct_North_95t07}
%\csname @@input\endcsname{inputs/north_subperiod/Results2ROB_ct_North_95t07}
%\csname @@input\endcsname{inputs/north_subperiod/Results2ICT_ct_North_95t07}
%\csname @@input\endcsname{inputs/north_subperiod/Results2RICT_ct_North_95t07}
\csname @@input\endcsname{inputs/north_subperiod/Results2RICTint_ct_North_95t07}
\bottomrule
    \end{tabular}\end{adjustbox} \\ }
    %\label{tab:regr_pre_tax_prod6}
        \scriptsize
   Notes: \sym{*}\(p<0.05\), \sym{**}\(p<0.01\), \sym{***}\(p<0.001\). Regression results to examine the link between tax aggregation and economic production for Northern European countries during the period 1995-2007. All regressions use country level data and include: GDP growth ($GDPgrowth_{c,t}$); share of gross output produced in service industries ($Services_{c,t}$); Herfindahl-Hirschman Index based on the gross output shares of macro-sectors ($HHI_{c,t}$); government consolidated gross debt as \% of GDP ($Debt^{\%GDP}_{c,t}$); government interest payable as \% of GDP ($Interest^{\%GDP}_{c,t}$); net government lending/borrowing as \% of GDP ($Lending^{\%GDP}_{c,t}$); gross fixed capital formation as \% of GDP ($GovInv^{\%GDP}_{c,t}$); period average exchange rate ($XRate_{c,t}$); and country ($c$) and year ($t$) fixed effects. For the first block (Taxes in ln of national currency), $wL_{c,t}$, $rK_{c,t}$ and $pQ_{c,t}$ are expressed as the natural logarithm ($ln$) while for the last two blocks they are expressed as \% of GDP.
    \end{table}
%    \end{landscape}

	\begin{table}[H]
	{\centering 
     
    \caption{Taxation and the structure of production in Northern Europe after 2008}
    \begin{adjustbox}{width=\textwidth}\begin{tabular}{l|cccc|cccc|ccc}
    \toprule \addlinespace
\csname @@input\endcsname{inputs/north_subperiod/Results2RICTint_ct_North_08t16}
\bottomrule
    \end{tabular}\end{adjustbox} \\ }
    %\label{tab:regr_pre_tax_prod6}
        \scriptsize
   Notes: \sym{*}\(p<0.05\), \sym{**}\(p<0.01\), \sym{***}\(p<0.001\). Regression results to examine the link between tax aggregation and economic production for Northern European countries during the period 2008-2016. All regressions use country level data and include: GDP growth ($GDPgrowth_{c,t}$); share of gross output produced in service industries ($Services_{c,t}$); Herfindahl-Hirschman Index based on the gross output shares of macro-sectors ($HHI_{c,t}$); government consolidated gross debt as \% of GDP ($Debt^{\%GDP}_{c,t}$); government interest payable as \% of GDP ($Interest^{\%GDP}_{c,t}$); net government lending/borrowing as \% of GDP ($Lending^{\%GDP}_{c,t}$); gross fixed capital formation as \% of GDP ($GovInv^{\%GDP}_{c,t}$); period average exchange rate ($XRate_{c,t}$); and country ($c$) and year ($t$) fixed effects. For the first block (Taxes in ln of national currency), $wL_{c,t}$, $rK_{c,t}$ and $pQ_{c,t}$ are expressed as the natural logarithm ($ln$) while for the last two blocks they are expressed as \% of GDP..
    \end{table}
%    \end{landscape}

\FloatBarrier

	\begin{table}[H]
	{\centering 
     
    \caption{Taxation and the structure of production in Southern Europe}
    \begin{adjustbox}{width=\textwidth}\begin{tabular}{l|cccc|cccc|ccc}
    \toprule \addlinespace
\csname @@input\endcsname{inputs/south_95_16/Results2RICTint_ct_South_95t16}
\bottomrule
    \end{tabular}\end{adjustbox} \\ }
    %\label{tab:regr_pre_tax_prod6}
        \scriptsize
   Notes: \sym{*}\(p<0.05\), \sym{**}\(p<0.01\), \sym{***}\(p<0.001\). Regression results to examine the link between tax aggregation and economic production for Southern European countries during the period 1995-2016. All regressions use country level data and include: GDP growth ($GDPgrowth_{c,t}$); share of gross output produced in service industries ($Services_{c,t}$); Herfindahl-Hirschman Index based on the gross output shares of macro-sectors ($HHI_{c,t}$); government consolidated gross debt as \% of GDP ($Debt^{\%GDP}_{c,t}$); government interest payable as \% of GDP ($Interest^{\%GDP}_{c,t}$); net government lending/borrowing as \% of GDP ($Lending^{\%GDP}_{c,t}$); gross fixed capital formation as \% of GDP ($GovInv^{\%GDP}_{c,t}$); period average exchange rate ($XRate_{c,t}$); and country ($c$) and year ($t$) fixed effects. For the first block (Taxes in ln of national currency), $wL_{c,t}$, $rK_{c,t}$ and $pQ_{c,t}$ are expressed as the natural logarithm ($ln$) while for the last two blocks they are expressed as \% of GDP.
    \end{table}
%    \end{landscape}

	\begin{table}[H]
	{\centering 
     
    \caption{Taxation and the structure of production in Southern Europe before 2007}
    \begin{adjustbox}{width=\textwidth}\begin{tabular}{l|cccc|cccc|ccc}
    \toprule \addlinespace
\csname @@input\endcsname{inputs/south_subperiod/Results2RICTint_ct_South_95t07}
\bottomrule
    \end{tabular}\end{adjustbox} \\ }
    %\label{tab:regr_pre_tax_prod6}
        \scriptsize
   Notes: \sym{*}\(p<0.05\), \sym{**}\(p<0.01\), \sym{***}\(p<0.001\). Regression results to examine the link between tax aggregation and economic production for Southern European countries during the period 1995-2007. All regressions use country level data and include: GDP growth ($GDPgrowth_{c,t}$); share of gross output produced in service industries ($Services_{c,t}$); Herfindahl-Hirschman Index based on the gross output shares of macro-sectors ($HHI_{c,t}$); government consolidated gross debt as \% of GDP ($Debt^{\%GDP}_{c,t}$); government interest payable as \% of GDP ($Interest^{\%GDP}_{c,t}$); net government lending/borrowing as \% of GDP ($Lending^{\%GDP}_{c,t}$); gross fixed capital formation as \% of GDP ($GovInv^{\%GDP}_{c,t}$); period average exchange rate ($XRate_{c,t}$); and country ($c$) and year ($t$) fixed effects. For the first block (Taxes in ln of national currency), $wL_{c,t}$, $rK_{c,t}$ and $pQ_{c,t}$ are expressed as the natural logarithm ($ln$) while for the last two blocks they are expressed as \% of GDP.
    \end{table}
%    \end{landscape}

	\begin{table}[H]
	{\centering 
     
    \caption{Taxation and the structure of production in Southern Europe after 2008}
    \begin{adjustbox}{width=\textwidth}\begin{tabular}{l|cccc|cccc|ccc}
    \toprule \addlinespace
\csname @@input\endcsname{inputs/south_subperiod/Results2RICTint_ct_South_08t16}
\bottomrule
    \end{tabular}\end{adjustbox} \\ }
    %\label{tab:regr_pre_tax_prod6}
        \scriptsize
   Notes: \sym{*}\(p<0.05\), \sym{**}\(p<0.01\), \sym{***}\(p<0.001\). Regression results to examine the link between tax aggregation and economic production for Southern European countries during the period 2008-2016. All regressions use country level data and include: GDP growth ($GDPgrowth_{c,t}$); share of gross output produced in service industries ($Services_{c,t}$); Herfindahl-Hirschman Index based on the gross output shares of macro-sectors ($HHI_{c,t}$); government consolidated gross debt as \% of GDP ($Debt^{\%GDP}_{c,t}$); government interest payable as \% of GDP ($Interest^{\%GDP}_{c,t}$); net government lending/borrowing as \% of GDP ($Lending^{\%GDP}_{c,t}$); gross fixed capital formation as \% of GDP ($GovInv^{\%GDP}_{c,t}$); period average exchange rate ($XRate_{c,t}$); and country ($c$) and year ($t$) fixed effects. For the first block (Taxes in ln of national currency), $wL_{c,t}$, $rK_{c,t}$ and $pQ_{c,t}$ are expressed as the natural logarithm ($ln$) while for the last two blocks they are expressed as \% of GDP.
    \end{table}
%    \end{landscape}

\FloatBarrier

\subsection{The economic impact of automation by region}
\label{appendix:add_results_ai_and_the_economy}
\subsubsection{The replacement effect}
\label{appendix:replacement_country}
	
	\textcolor{red}{check these}
	
	In Eastern Europe, we find robots and the depth of automation to coincide with labor replacement reflected in lower employment. The effects on capital prices are ambiguous: ICT ($R \ast ICT_{i,c,t}$) exhibits negative (positive) correlations with $r_{i,c,t}$. These relationships are more prevalent before 2007. 
	
	In Northern Europe and after 2008, we observe a replacement effect reflected in a decreasing wage bill and labor demand induced by robots. During that period, we also observe that ICT diffusion is associated with lower labor demand. Prior to 2007, we observe almost no significant effects. We only find a positive correlation of robot diffusion and capital accumulation. 
	
	In Southern Europe, we do not observe any AT-induced replacement effect. ICT is positively correlated with the wage bill throughout all periods. While we do not find any effect of robots on labor demand, we see that robot diffusion is associated with increasing wages. 
	ICT and the depth of automation are both associated with increasing capital prices but decreasing capital stocks. 

			\begin{table}[H]
    {\centering 
    \caption{The replacement effect in Eastern Europe}
    %\label{tab:regr_replacement_east}
    \begin{adjustbox}{width=0.8\textwidth}\begin{tabular}{l|ccc|ccc}
    %\begin{adjustbox}{width=\textwidth}\begin{tabular}{p{0.6cm}|p{.95cm}p{.95cm}p{.95cm}|p{.95cm}p{.95cm}p{.95cm}|p{.95cm}p{.95cm}p{.95cm}|p{.95cm}p{.95cm}p{.95cm}}
    \toprule \addlinespace
    
    \csname @@input\endcsname{inputs/east_95_16/Results3RICTint_cit_East_95t16}

    \bottomrule \addlinespace
%\multicolumn{13}{l}{\emph{\underline{Sub-period from 1995 to 2007}}}\\ %\addlinespace
\csname @@input\endcsname{inputs/east_subperiod/Results3RICTint_cit_East_95t07}

\bottomrule \addlinespace
%\multicolumn{13}{l}{\emph{\underline{Sub-period from 1995 to 2007}}}\\ %\addlinespace
\csname @@input\endcsname{inputs/east_subperiod/Results3RICTint_cit_East_08t16}
\bottomrule
    \end{tabular}\end{adjustbox}\\ }
    \scriptsize
    Notes: \sym{*}\(p<0.05\), \sym{**}\(p<0.01\), \sym{***}\(p<0.001\). Regression results to test the replacement effect for Eastern European countries during the period 1995-2016. All regressions use industry level data for the subset of industries susceptible to automation, defined as industries were the use of industrial robots is prevalent (see Appendix Table~\ref{appendix:data}). All regressions include: country industry ($ci$); country year ($ct$); and industry year ($it$) fixed effects. All regressions are weighted by the base-sample-year share of each industry’s number of hours worked to country-wide hours worked.
    \end{table}
\FloatBarrier
			\begin{table}[H]
    {\centering 
    \caption{The replacement effect in Northern Europe}
    %\label{tab:regr_replacement_north}
    \begin{adjustbox}{width=0.8\textwidth}\begin{tabular}{l|ccc|ccc}
    %\begin{adjustbox}{width=\textwidth}\begin{tabular}{p{0.6cm}|p{.95cm}p{.95cm}p{.95cm}|p{.95cm}p{.95cm}p{.95cm}|p{.95cm}p{.95cm}p{.95cm}|p{.95cm}p{.95cm}p{.95cm}}
    \toprule \addlinespace
    
    \csname @@input\endcsname{inputs/north_95_16/Results3RICTint_cit_North_95t16}

    \bottomrule \addlinespace
%\multicolumn{13}{l}{\emph{\underline{Sub-period from 1995 to 2007}}}\\ %\addlinespace
\csname @@input\endcsname{inputs/north_subperiod/Results3RICTint_cit_North_95t07}

\bottomrule \addlinespace
%\multicolumn{13}{l}{\emph{\underline{Sub-period from 1995 to 2007}}}\\ %\addlinespace
\csname @@input\endcsname{inputs/north_subperiod/Results3RICTint_cit_North_08t16}
\bottomrule
    \end{tabular}\end{adjustbox}\\ }
    \scriptsize
    Notes: \sym{*}\(p<0.05\), \sym{**}\(p<0.01\), \sym{***}\(p<0.001\). Regression results to test the replacement effect for Northern European countries during the period 1995-2016. All regressions use industry level data for the subset of industries susceptible to automation, defined as industries were the use of industrial robots is prevalent (see Appendix Table~\ref{appendix:data}). All regressions include: country industry ($ci$); country year ($ct$); and industry year ($it$) fixed effects. All regressions are weighted by the base-sample-year share of each industry’s number of hours worked to country-wide hours worked.
    \end{table}
\FloatBarrier
			\begin{table}[H]
    {\centering 
    \caption{The replacement effect in Southern Europe}
    %\label{tab:regr_replacement_south}
    \begin{adjustbox}{width=0.8\textwidth}\begin{tabular}{l|ccc|ccc}
    %\begin{adjustbox}{width=\textwidth}\begin{tabular}{p{0.6cm}|p{.95cm}p{.95cm}p{.95cm}|p{.95cm}p{.95cm}p{.95cm}|p{.95cm}p{.95cm}p{.95cm}|p{.95cm}p{.95cm}p{.95cm}}
    \toprule \addlinespace
    
    \csname @@input\endcsname{inputs/south_95_16/Results3RICTint_cit_South_95t16}

    \bottomrule \addlinespace
%\multicolumn{13}{l}{\emph{\underline{Sub-period from 1995 to 2007}}}\\ %\addlinespace
\csname @@input\endcsname{inputs/south_subperiod/Results3RICTint_cit_South_95t07}

\bottomrule \addlinespace
%\multicolumn{13}{l}{\emph{\underline{Sub-period from 1995 to 2007}}}\\ %\addlinespace
\csname @@input\endcsname{inputs/south_subperiod/Results3RICTint_cit_South_08t16}
\bottomrule
    \end{tabular}\end{adjustbox}\\ }
    \scriptsize
    Notes: \sym{*}\(p<0.05\), \sym{**}\(p<0.01\), \sym{***}\(p<0.001\). Regression results to test the replacement effect for Southern European countries during the period 1995-2016. All regressions use industry level data for the subset of industries susceptible to automation, defined as industries were the use of industrial robots is prevalent (see Appendix Table~\ref{appendix:data}). All regressions include: country industry ($ci$); country year ($ct$); and industry year ($it$) fixed effects. All regressions are weighted by the base-sample-year share of each industry’s number of hours worked to country-wide hours worked.
    \end{table}
\FloatBarrier

\subsubsection{The reinstatement effect}
\label{appendix:reinstatement_country}
In Eastern Europe, we find robots to exhibit a negative association with country level wages and capital prices, but a positive one with total employment. 
For ICT, we observe the opposite pattern, i.e. increasing wages and capital prices. Effects on factor demand for labor and capital are not significant. 
We find that robots are correlated with increasing wage inequality and ICT with a decreasing output share of services. 

In Northern Europe, we do not find any support for a robot induced reinstatement effect: The diffusion of robots exhibits a negative association with factor prices and quantities for both, capital and labor. We also find that robot diffusion is associated with a decline in services. 
For ICT diffusion, we find almost no significant effects. We only observe an increasing output share of services after 2008. 

		\begin{table}[H]
    {\centering 
    \caption{The reinstatement effect in Eastern Europe}
    %\label{tab:regr_reinstatement}
    \begin{adjustbox}{width=\textwidth}\begin{tabular}{l|ccccccc}
    %\begin{adjustbox}{width=\textwidth}\begin{tabular}{p{0.6cm}|p{.95cm}p{.95cm}p{.95cm}|p{.95cm}p{.95cm}p{.95cm}|p{.95cm}p{.95cm}p{.95cm}|p{.95cm}p{.95cm}p{.95cm}}
    \toprule \addlinespace

\csname @@input\endcsname{inputs/east_95_16/Results4shortRICTint_ct_East_95t16}
\bottomrule \addlinespace
\csname @@input\endcsname{inputs/east_subperiod/Results4shortRICTint_ct_East_95t07}
\bottomrule \addlinespace
\csname @@input\endcsname{inputs/east_subperiod/Results4shortRICTint_ct_East_08t16}
\bottomrule
    \end{tabular}\end{adjustbox}\\ }
    \scriptsize
    Notes: \sym{*}\(p<0.05\), \sym{**}\(p<0.01\), \sym{***}\(p<0.001\). Regression results to test the reinstatement effect for Eastern European countries during the period 1995-2016. All regressions include: GDP growth, government consolidated gross debt as \% of GDP; government interest payable as \% of GDP; net government lending/borrowing as \% of GDP; gross fixed capital formation as \% of GDP; period average exchange rate; value added TFP--calculated as the residual from an OLS regression of value-added volumes ($VA$) on a translog production function including capital volumes ($K$) and total number of hours worked ($L$); and country ($c$) and year ($t$) fixed effects.
    
    \end{table}

\FloatBarrier

		\begin{table}[H]
    {\centering 
    \caption{The reinstatement effect in Northern Europe}
    %\label{tab:regr_reinstatement}
    \begin{adjustbox}{width=\textwidth}\begin{tabular}{l|ccccccc}
    \toprule \addlinespace

\csname @@input\endcsname{inputs/north_95_16/Results4shortRICTint_ct_North_95t16}
\bottomrule \addlinespace
\csname @@input\endcsname{inputs/north_subperiod/Results4shortRICTint_ct_North_95t07}
\bottomrule \addlinespace
\csname @@input\endcsname{inputs/north_subperiod/Results4shortRICTint_ct_North_08t16}
\bottomrule
    \end{tabular}\end{adjustbox}\\ }
    \scriptsize
    Notes: \sym{*}\(p<0.05\), \sym{**}\(p<0.01\), \sym{***}\(p<0.001\). Regression results to test the reinstatement effect for Northern European countries during the period 1995-2016. All regressions include: GDP growth, government consolidated gross debt as \% of GDP; government interest payable as \% of GDP; net government lending/borrowing as \% of GDP; gross fixed capital formation as \% of GDP; period average exchange rate; value added TFP--calculated as the residual from an OLS regression of value-added volumes ($VA$) on a translog production function including capital volumes ($K$) and total number of hours worked ($L$); and country ($c$) and year ($t$) fixed effects.
    
    \end{table}

\FloatBarrier

		\begin{table}[H]
    {\centering 
    \caption{The reinstatement effect in Southern Europe}
    %\label{tab:regr_reinstatement}
    \begin{adjustbox}{width=\textwidth}\begin{tabular}{l|ccccccc}
    \toprule \addlinespace

\csname @@input\endcsname{inputs/south_95_16/Results4shortRICTint_ct_South_95t16}
\bottomrule \addlinespace
\csname @@input\endcsname{inputs/south_subperiod/Results4shortRICTint_ct_South_95t07}
\bottomrule \addlinespace
\csname @@input\endcsname{inputs/south_subperiod/Results4shortRICTint_ct_South_08t16}
\bottomrule
    \end{tabular}\end{adjustbox}\\ }
    \scriptsize
    Notes: \sym{*}\(p<0.05\), \sym{**}\(p<0.01\), \sym{***}\(p<0.001\). Regression results to test the reinstatement effect for Southern European countries during the period 1995-2016. All regressions include: GDP growth, government consolidated gross debt as \% of GDP; government interest payable as \% of GDP; net government lending/borrowing as \% of GDP; gross fixed capital formation as \% of GDP; period average exchange rate; value added TFP--calculated as the residual from an OLS regression of value-added volumes ($VA$) on a translog production function including capital volumes ($K$) and total number of hours worked ($L$); and country ($c$) and year ($t$) fixed effects.
    
    \end{table}

\FloatBarrier

\subsubsection{The real income effect}
\label{appendix:real_income_country}
For the subset of Eastern European countries, we find that robot diffusion is significantly negatively correlated with factor incomes, both capital and labor. We find a negative impact on prices, but observe an expansion of output. 
ICT exhibits only a weak negative correlation with prices and TFP, and prior to 20017, we also observe a negative association with capital income. 

In Norther Europe, we observe similar patterns, i.e. negative correlations between robot diffusion and factor revenues and output prices. For ICT and the depth of automation, we do not find any significant effects. 

The patterns in Southern Europe are different: After 2008, we find that robots are significantly positively related to labor and capital income and to output and sales. WE also observe a positive correlation with TFP.  
	
	\begin{table}[H]
    {\centering 
        \caption{The real income effect in Eastern Europe}
            %\label{tab:regr_realincome_east_9516}

    \begin{adjustbox}{width=\textwidth}\begin{tabular}{l|cccccccc}
    \toprule \addlinespace
\csname @@input\endcsname{inputs/east_95_16/Results5RICTint_ct_East_95t16}
\bottomrule \addlinespace
\csname @@input\endcsname{inputs/east_subperiod/Results5RICTint_ct_East_95t07}
\bottomrule \addlinespace
\csname @@input\endcsname{inputs/east_subperiod/Results5RICTint_ct_East_08t16}
\bottomrule
    \end{tabular}\end{adjustbox}\\ \noindent }
    \scriptsize
    Notes: \sym{*}\(p<0.05\), \sym{**}\(p<0.01\), \sym{***}\(p<0.001\). Regression results to test the real income effect for Eastern European countries during the period 1995-2016. Labor productivity is measured as the share of gross output volumes ($Q$) over the total number of hours worked. TFP is calculated as the residual from an OLS regression of gross output volumes ($Q$) on a translog production function including capital volumes ($K$), total number of hours worked ($L$) and intermediate input volumes ($M$). All regressions include: GDP growth, government consolidated gross debt as \% of GDP; government interest payable as \% of GDP; net government lending/borrowing as \% of GDP; gross fixed capital formation as \% of GDP; period average exchange rate; and country ($c$) and year ($t$) fixed effects.
    \end{table}

\FloatBarrier
	\begin{table}[H]
    {\centering 
        \caption{The real income effect in Northern Europe}
            %\label{tab:regr_realincome_north_9516}

    \begin{adjustbox}{width=\textwidth}\begin{tabular}{l|cccccccc}
    \toprule \addlinespace
\csname @@input\endcsname{inputs/north_95_16/Results5RICTint_ct_North_95t16}
\bottomrule \addlinespace
\csname @@input\endcsname{inputs/north_subperiod/Results5RICTint_ct_North_95t07}
\bottomrule \addlinespace
\csname @@input\endcsname{inputs/north_subperiod/Results5RICTint_ct_North_08t16}
\bottomrule
    \end{tabular}\end{adjustbox}\\ \noindent }
    \scriptsize
    Notes: \sym{*}\(p<0.05\), \sym{**}\(p<0.01\), \sym{***}\(p<0.001\). Regression results to test the real income effect for Northern European countries during the period 1995-2016. Labor productivity is measured as the share of gross output volumes ($Q$) over the total number of hours worked. TFP is calculated as the residual from an OLS regression of gross output volumes ($Q$) on a translog production function including capital volumes ($K$), total number of hours worked ($L$) and intermediate input volumes ($M$). All regressions include: GDP growth, government consolidated gross debt as \% of GDP; government interest payable as \% of GDP; net government lending/borrowing as \% of GDP; gross fixed capital formation as \% of GDP; period average exchange rate; and country ($c$) and year ($t$) fixed effects.
    \end{table}

\FloatBarrier

	\begin{table}
    {\centering 
        \caption{The real income effect in Southern Europe}
            %\label{tab:regr_realincome_south_9516}

    \begin{adjustbox}{width=\textwidth}\begin{tabular}{l|cccccccc}
    \toprule \addlinespace
\csname @@input\endcsname{inputs/south_95_16/Results5RICTint_ct_South_95t16}
\bottomrule \addlinespace
\csname @@input\endcsname{inputs/south_subperiod/Results5RICTint_ct_South_95t07}
\bottomrule \addlinespace
\csname @@input\endcsname{inputs/south_subperiod/Results5RICTint_ct_South_08t16}
\bottomrule
    \end{tabular}\end{adjustbox}\\ \noindent }
    \scriptsize
    Notes: \sym{*}\(p<0.05\), \sym{**}\(p<0.01\), \sym{***}\(p<0.001\). Regression results to test the real income effect for Southern European countries during the period 1995-2016. Labor productivity is measured as the share of gross output volumes ($Q$) over the total number of hours worked. TFP is calculated as the residual from an OLS regression of gross output volumes ($Q$) on a translog production function including capital volumes ($K$), total number of hours worked ($L$) and intermediate input volumes ($M$). All regressions include: GDP growth, government consolidated gross debt as \% of GDP; government interest payable as \% of GDP; net government lending/borrowing as \% of GDP; gross fixed capital formation as \% of GDP; period average exchange rate; and country ($c$) and year ($t$) fixed effects.
    \end{table}

\section{Analysis at the sub-national level}
\label{SM:firm_level}
The impact of automation is heterogeneous across firms, industries and regions. 
To analyze the impact of automation on aggregate taxation, we would ideally have data that provides a direct link between firm and industry level production accounts and tax payments. 
%that can be aggregated to see impact of automation on the revenue side of governments' budgets. 
But this data does not exist and granular data on firm or industry level tax payments draws only a partial picture: For example, at the firm level we have data on corporate taxes charged on profits and represent a part of aggregate taxes on capital. But we do not know how profits of individual firms or industries affect individual wealth levels and the demand for saving, investment in financial accounts and durable goods (e.g. housing) which all are subject to other kinds of taxation. 

We complement the macro level analysis with a region level approach using firm level data provided by \citet{BvD2020data} and analyze the nexus between regional patterns of automation, labor demand and corporate tax payments in NUTS2-regions. This analysis draws only a partial picture of economic reality, but illustrates that the impacts of automation are diverse at the granular level. For governments, this understanding is important because --- dependent on the country-specific structure of tax administration --- locally raised taxes can be decisive to ensure the financing of essential public infrastructure. 

\subsection{Empirical approach}
	\label{SM:empirical_local_analysis}
	%The impact of ATs is heterogeneous across firms and industries. In the analyses described above, we study its effect on the structure of economic production and taxation at the national level. 
    But as explained in Sec. \ref{sec:background_taxation}, tax revenues are collected at different levels of government administration (central, federal, local).  
    For governments it is also relevant to understand the impact of automation at the local level. 
    To analyze the local effects of automation, we would ideally use regional data on economic production, automation and taxation. Unfortunately, this data is not available in a format that is consistent with the country level analysis introduced above. 
    
    As an alternative, we use firm level data being aware that firm level evidence draws only a partial picture of the economic reality. 
    In particular, we rely on the proprietary firm level data set Amadeus, the European counterpart of ORBIS-Global, which is a product of \citet{BvD2020data} (BvDEP). The underlying data are firms' financial statements sourced from various national registries (e.g. statistical agencies) and standardized by BvDEP for cross-country comparability.\footnote{For more details over the standardization procedure, see the correspondence tables used for each country by \citet{BvD2020manual}. 
    For the initial data cleaning and preparation procedure we follow \cite{kalemli2015construct}. Specifically, we drop firms reporting consolidated accounts, i.e. C1 and C2 codes and, if duplicate, the rest is kept based on the presence of annual reports over local registry filling. We also use annual records over quarters and late calendar months over early months.}
    
    For the analysis, we rely on balance sheet information of firms in the European countries where the industry level information on robot- or ICT-intensity exist for the period 2008-2016. To cover the largest set of regions across EU possible, we examine the effects of robot- and ICT-intensity separately and, thus, rely on the maximal amount of information available across data sets. More precisely, the sample used to analyze the impact of ICT-intensity ($ICT_{i,c,t}$) covers the same set of countries and industries used in the country  and industry level analysis from above. The sample used to analyze the impact of robot-intensity ($R_{i,c,t}$) also includes the following set of countries: Croatia (HR); Hungary (HU); Ireland (IE); Poland (PL); Portugal (PT); and Romania (RO).
    
    For each firm in the data set we retain those reporting strictly positive firm-year values on the number of employees or taxes payed. The latter refers to income tax expenses of the reporting period plus any net deferred tax expenses/income between the current and the previous reporting period. Conclusions drawn from this analysis are limited to a rather specific category of fiscal taxes, i.e. corporate income taxes.
    
    Each firm's primary production activity is based on the NACE Rev.2 (ISIC Rev.4) 2-digit industry code used to merge with the industry level measures on robot- and ICT-intensity.
    The sample includes the same set of 15 industry groups covered in the industry level sample (see Appendix Table~\ref{tab:industry_codes} for a detailed description of the industry codes). Finally, we link firms to the location of economic activity trough the NUTS version 2016 regional classification codes which across the EU and UK cover 281 regions at NUTS 2 and 1348 regions at NUTS 3 level \citep{eurostat2020nuts}. The sample used in our analysis for the effects of robot (ICT) intensity covers 273 (227) NUTS 2 and 1314 (1127) NUTS 3 regions. For more details over the summary statistics of the firm level sample and variables considered, see Appendix Table~\ref{tab:descriptives_firm}.

    ORBIS-Global is widely accepted as one of the best available options in terms of the richness of balance sheet information and cross-country comparability at the expense of incomplete coverage for smaller-sized firms with simplified financial reporting obligations \citep{bajgar2020coverage,kalemli2015construct}. Thus, while a large number of micro firms remain unrecorded, the sample manages to cover around 60\% of economic activity in terms of employment, on average (see Appendix Table~\ref{tab:coverage_firm_L}).\footnote{For similar evidence see \citet{bormans2020link}.}
    
    However, it is still crucial to understand the representativeness of the firm level corporate income taxes relative to the economy wide capital and corporate income taxes. Even when we look at the country level sample, we find that corporate taxes on income, profits and capital gains (variable code 1200 in \citet{OECD2019} data set) represent only 22\% of total capital taxes $T^{k}$, on average across sample-countries (see Appendix Table~\ref{tab:coverage_firm_T}). When we focus on the firm level samples we see that, on average, they represent around 20\% of the economy-wide corporate taxes on income, profits and capital gains (see Appendix Table~\ref{tab:coverage_firm_T}). This gap is mainly driven by the fact that in the firm level samples we only observe firms in the limited sub-set of the 15 industry groupings used in the industry level analysis and not the whole economy. However, even if we observed firm level data for the whole economy the sample will remain underrepresented, in line with the results from above on the coverage on employment. Overall, while the firm level data is helpful in uncovering interesting underlying heterogeneity, any results will capture a very limited part of the aggregate effects.
    
    Using a regression analysis, we estimate the impact of robot $R_{i,c,t}$ and $ICT_{i,c,t}$ intensity on regional labor demand $L_{f,r,i,t}$ and corporate tax payment $T^{\pi}_{f,r,i,t}$. To illustrate the effects, we estimate for each country the following specification
    \begin{equation}
        Y_{f,r,t} \sim \beta^{x}_{r} \cdot \mathbbm{1}(r,i)_f \cdot X_{i,c,t} + \epsilon_{r,f,t}
    \end{equation}
    where $Y_{f,r,t} \in \{ T^{\pi}_{f,r,t}, L_{f,r,t} \}$, $X_{i,c,t} \in \{ R_{i,c,t}, ICT_{i,c,t}\}$ and $i \in I_c$. $\mathbbm{1}(r,i)_f$ is a firm-specific dummy variable that equals one if firm $f$ is located in region $r$ and with primary economic activity in industry $i$.\footnote{Since we drop firms reporting consolidated accounts, we account for any double counting that could possibly arise from subsidiary firms integrating their statements to the national of international headquarter. However, we cannot control for such a possibility for multi-plant firms, due to the absence of data at such granular level.} All regressions include firm and NUTS3-region-year FE and are weighted using the same weights as in the industry level analysis, i.e. base-sample-year share of each industry’s number of hours worked to country-wide hours worked. For the standard errors, we use multi-way clustering at the industry, region and year level.
    
    Note that we combine data from different levels of aggregation here. In particular, we merge industry-country level data on automation with firm level data where the location of the firm is observed. This way we are able to map the industry-country level to the region-level dimension. However, since we do not directly observe the allocation of robot and ICT-intensity across regions, our estimation strategy assumes that all industries within an country are equally exposed to automation independent of the regional identity. Using this estimation strategy, we capture within-industry technological change and induced reallocation across firms that might be regionally unequally distributed.%\footnote{\green{@A: Moreover, do we use weights in the end? This should be mentioned here. Some general remark, not sure whether we should act on this, but we should think about reasons for our decision: Above, we have included R and ICT simultaneously. Why don't we do this here? I would not re-do the analysis, but we should be able to provide arguments (if a reviewer is asking for this, at least I would ask for this).} \textcolor{red}{@K and P: We use the same industry level weights as in the industry level analysis. Concerning the reasoning on why we do not include it simultaneously, I briefly discuss it above in the data section. The general idea is that Robot intensity is available for an additional 5 countries and thus we want to explore most of regions available.} \green{K@A: My question was related to the question whether we use firm-specific weight capturing the weight of a firm within and industry and the weight of an industry within a country simultaneously. In my view, still the best approach content-wise, but I suggest to do this only, if any reviewer is complaining about this. The firm level analysis is too limited in many other regards such that I find it is not worth the effort to spend more time on this.}} 
    
    We illustrate the effects of ICT and robot adoption at the regional level drawing maps that show the estimated effect $\beta_{r}$ on corporate taxes and on local labor demand. Different color codes indicate the size and direction of the expected impact.

	\FloatBarrier

\subsection{Results}
\label{SM:results_local_analysis}
In the preceding analysis, we observed that the economic effects of automation can be heterogeneous across different groups of countries. This indicates that local conditions matter. Now, we explore regional heterogeneity at the sub-national level. 

In Fig. \ref{fig:ai_nuts2}, we show the regional effects of automation at the level of NUTS2 regions. The figures on top (Fig. \ref{fig:nuts2_LR} and \ref{fig:nuts2_LICT}) show the effects on local labor demand that is captured by the firms in our sample. The figures at the bottom illustrate the correlation between automation and corporate tax revenues (Fig. \ref{fig:nuts2_TR} and \ref{fig:nuts2_TICT}). On the left (right) hand side, we show the estimated effects of robot (ICT) adoption. The colors indicate the scale of the effect where green color indicates positive and red color negative estimated effects. 
Additional plots at the NUTS3 and at the country level aggregated from firm level data are available in the Appendix \ref{appendix:add_results_local_effects}. 

Visually, indicated by the similar coloring patterns comparing the map at the top with its analog at the bottom, it can be seen that in most regions the effects of automation on labor and taxation point into the same direction: When ATs exhibit a negative association with employment, we also observe a negative impact with corporate tax payments. Few exceptions at the local level exist where we find an opposite pattern of correlation. For example, in Alentejo (Portugal, PT18) and in Corse (France, FR83) the impact of robots on labor is negatively correlated with its impact on corporate taxes. In parts of Ireland and many regions of the UK, we observe generally a negative correlation between the effect of robots on tax revenues and on labor as indicated by opposite coloring codes for each NUTS regions, i.e. robots have a negative impact on labor but a positive impact on corporate tax payments and vice versa. 
% Note for interpretation: This could be due to distributional issues (for example, when robots come, many employment-intensive, but unproductive firms exit the market and high-profit-superstars with low employment grow) but it can be also due to design of fiscal policies. And many other explanations possible, recall industry level data and also cross-industry reallocation possible. 

We also observe that the impact of robots compared to ICT differs across regions and countries. For example, we observe robots to have a positive impact on labor and taxation in Italy, but we find a negative impact of ICT. The opposite pattern holds true for parts of Greece where ICT tends to exhibit a positive effect, but robots a negative one. 

Generally, we find that most regions in Spain, France and the Baltic countries to be the beneficiaries of automation: Both, robots and ICT diffusion, exhibit positive effects on regional labor demand and corporate taxation. The estimated effects draw a mixed picture of Germany and the UK: Some regions exhibit strong negative, others strong positive impacts. In Sweden and Finland, we find negative effects of robot diffusion on both, labor and taxes, and mixed effects of ICT. 

\begin{figure}
    {\centering
    
    \caption{Automation at the sub-national level (NUTS2 regions)}
    \label{fig:ai_nuts2}
    \begin{subfigure}[r]{0.49\textwidth}
    \subcaption{Labor \& robots}
     \label{fig:nuts2_LR}
     \includegraphics[width=\textwidth]{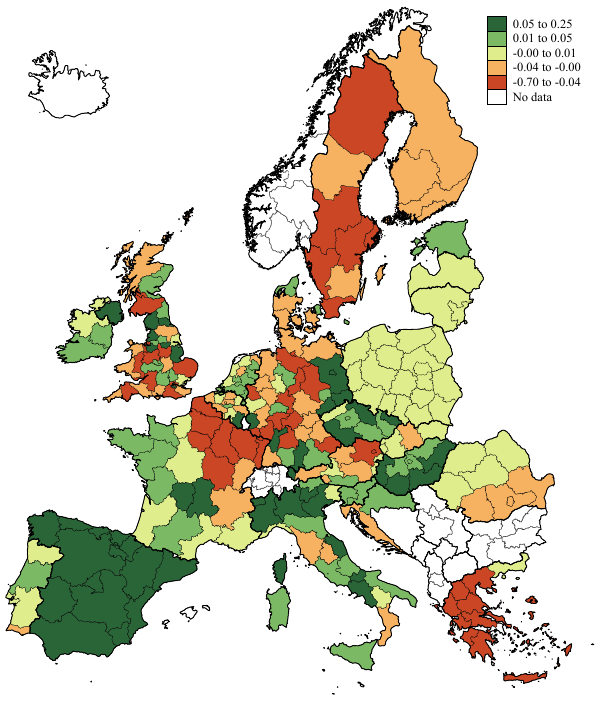}
    \end{subfigure}
        \begin{subfigure}[r]{0.49\textwidth}
        \subcaption{Labor \& ICT}
         \label{fig:nuts2_LICT}
     \includegraphics[width=\textwidth]{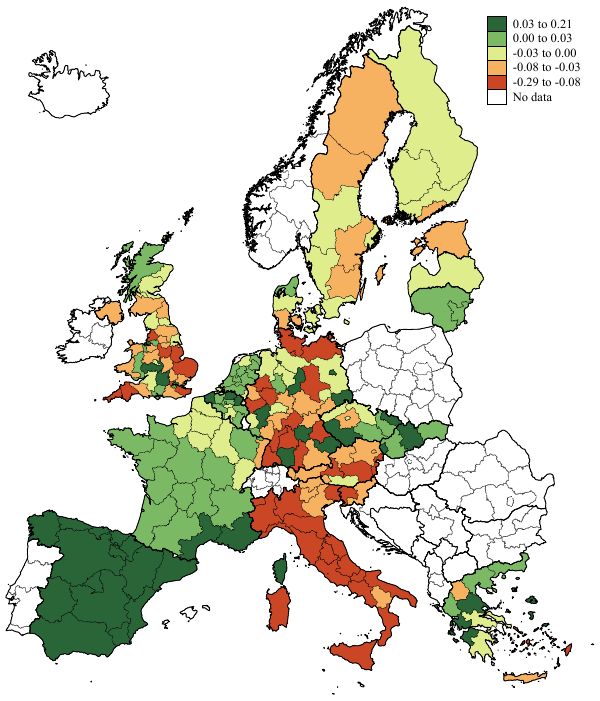}
    \end{subfigure}
    
    \begin{subfigure}[r]{0.49\textwidth}
    \subcaption{Taxes \& robots}
    \label{fig:nuts2_TR}
     \includegraphics[width=\textwidth]{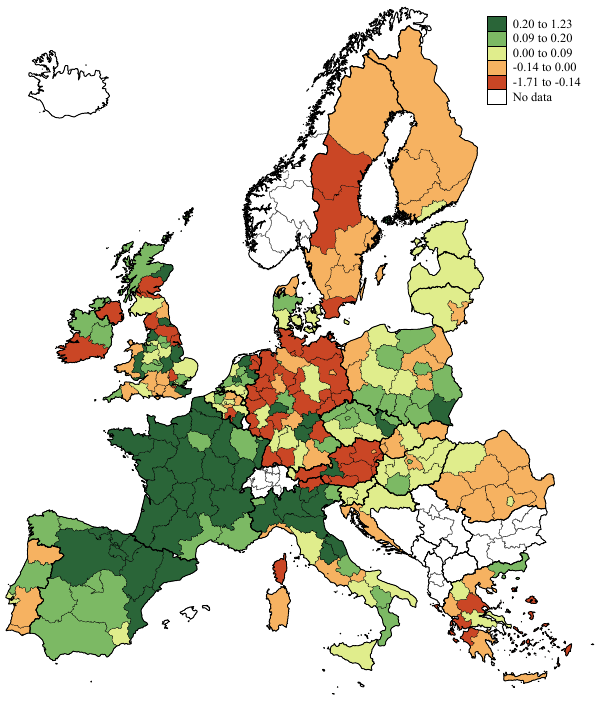}
    \end{subfigure}
    \begin{subfigure}[r]{0.49\textwidth}
    \subcaption{Taxes \& ICT}
    \label{fig:nuts2_TICT}
     \includegraphics[width=\textwidth]{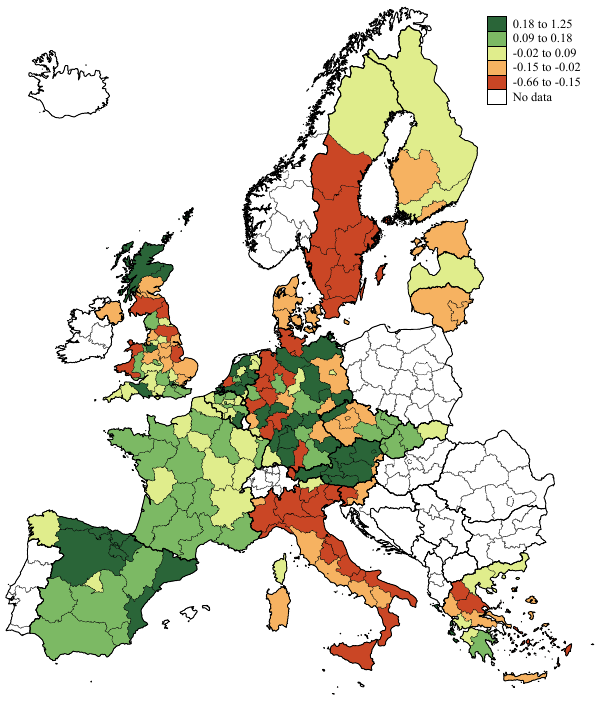}
     
    \end{subfigure}}
    \footnotesize
     \scriptsize
	    Source: Author's calculations based on ORBIS Global, IFR and EUKLEMS data sets.\\
	    Notes: Each map presents the point estimates from regressing for each country separately the ln of the firm level corporate income tax ($Taxes$) and number of employees ($L$), respectively, on the industry level robot ($R$) or $ICT$ intensity interacted with a full set of NUTS2 version 2016-regional dummies. All regressions include firm and NUTS3 version 2016-region-year fixed effects and are weighted using the same weights as in the industry level analysis, i.e. base-sample-year share of each industry’s number of hours worked to country-wide hours worked. The estimated effects are plotted with 2 shades of green and red for two groups of positive and negative values, respectively, with the darker colors representing stronger effects. Regions with no data are left blank. Panels (a) and (c) cover 273 NUTS2 regions, while panels (b) and (d) cover 227 NUTS2 regions.
\end{figure}

\FloatBarrier	

\subsection{Discussion and insights}
	Our analysis at the sub-national (NUTS2) level underlines the heterogeneity of impacts in two regards: (1) The linkage between economic outcomes, taxes to automation, and (2) the relationship between economic outcomes and tax payments differ across regions. Limited to corporate taxation in the period 2008-2016 and covering only a subset of industries and firms, we find that automation is positively correlated with employment in some regions, while negatively in others. 
	In most regions, we find a positive correlation between employment and taxes: Hence, when the net of the replacement and reinstatement effect is employment increasing, corporate tax payments tend to be higher. However, this relationship is reverse for some of the regions in our analysis. 
	Note that the sub-national analysis draws only a partial picture of the aggregate reality: Due to data limitations, we cover only corporate tax payments of a subset of firms drawn from a subset of industries. Corporate tax payments are a subset of capital taxes and represent only a fraction of total taxation. Hence, the results can not be extrapolated to the flows of aggregate taxation.
	%\footnote{\textcolor{red}{@A: Here it would be nice to have a number, i.e. (1) aggr. corporate taxes (covered by our data) over (1) $T^k$ and (2) $T^{total}$. You can use the average across countries, but if this is not too much effort, it would be also nice to see it country-wise which can be also an indicator how well our regional analysis represents a country.}}

\subsection{Additional information on firm level data}

\subsubsection{Data and descriptives}
		\begin{table}[H]
	 \caption{Representativeness of employment in ORBIS vs. EUKLEMS data}
        \label{tab:coverage_firm_L}
        {\centering
        %\begin{adjustbox}{width=\textwidth}
        \begin{tabular}{lccccc}
        \toprule
          & (1) & (2) & (3) & (4) & (5) \\                                  
 Country &\multicolumn{3}{c}{Total employment} & \multicolumn{2}{c}{Employment share \%} \\\cmidrule(r){2-4} \cmidrule(r){5-6}                                                  & EUKLEMS & $R$-sample & $ICT$-sample & $R$-sample & $ICT$-sample \\\midrule
AT          &   1,254,090&     932,795&     932,795&       74.38&       74.38\\
BE          &   1,130,893&     784,687&     784,687&       69.39&       69.39\\
CZ          &   2,080,420&   1,283,846&   1,283,846&       61.71&       61.71\\
DE          &  12,381,000&   8,997,709&   8,997,709&       72.67&       72.67\\
DK          &     733,000&     297,891&     297,891&       40.64&       40.64\\
EE          &     241,000&      57,452&      10,524&       23.84&        4.37\\
ES          &   4,787,000&   1,572,781&   1,572,781&       32.86&       32.86\\
FI          &     705,900&     824,132&     824,132&      116.75&      116.75\\
FR          &   6,386,000&   1,508,347&   1,508,347&       23.62&       23.62\\
GR          &     777,160&      49,835&      49,835&        6.41&        6.41\\
HR          &     545,340&     291,881&          N/A&       53.52&          N/A\\
HU          &   1,495,220&     536,044&          N/A&       35.85&          N/A\\
IE          &     472,790&     677,391&          N/A&      143.28&          N/A\\
IT          &   6,534,000&   4,614,803&   4,614,803&       70.63&       70.63\\
LT          &     495,570&     482,602&     294,167&       97.38&       59.36\\
LV          &     291,860&     113,203&     113,203&       38.79&       38.79\\
NL          &   1,654,000&   1,610,159&   1,610,159&       97.35&       97.35\\
PL          &   5,863,800&   1,313,027&          N/A&       22.39&          N/A\\
PT          &   1,389,160&     598,185&          N/A&       43.06&          N/A\\
RO          &   2,907,400&   1,470,350&          N/A&       50.57&          N/A\\
SE          &   1,489,000&   1,352,279&   1,352,279&       90.82&       90.82\\
SI          &     325,680&     155,516&      53,275&       47.75&       16.36\\
SK          &     821,310&     436,482&     436,482&       53.14&       53.14\\
UK          &   6,433,010&   4,806,876&   4,806,876&       74.72&       74.72\\\midrule
Mean        &   2,549,775&   1,448,678&   1,641,322&       60.06&       55.78\\

         \bottomrule
        \end{tabular}
        %\end{adjustbox}
        }\\
       \scriptsize
        Notes: Columns (1), (2) and (3) show the total number of employees in EUKLEMS, $R$-sample and $ICT$-sample, respectively, for each country in the last sample period, i.e. 2016.  $R$- and $ICT$-sample refer to the firm level ORBIS sample when robot- and ICT-density is reported, respectively. Columns (4) and (5) report the employment shares in \% covered by the firm level sample relative to the aggregate data in EUKLEMS, i.e. the ratio of (2) over (1) and (3) over (1), respectively. All samples cover the same 15 industry-groupings used in the analysis and discussed in detail in Appendix Table~\ref{tab:industry_codes}. 
    \end{table}
    
		\begin{table}[H]
	 \caption{Representativeness of corporate taxes in ORBIS firm level samples vs. OECD country level data.}
        \label{tab:coverage_firm_T}
        {\centering
        \begin{adjustbox}{width=0.8\textwidth}
        \begin{tabular}{lccccc}
        \toprule
          & (1) & (2) & (3) & (4) & (5) \\                                  Country &\multicolumn{3}{c}{Aggregate Tax} & \multicolumn{2}{c}{Tax share (Sample Tax/$T^{k,corp}_{c}$)\%} \\\cmidrule(r){2-4} \cmidrule(r){5-6}                                                  & $T^{k}_{c}$ & $T^{k,corp}_{c}$ & $T^{k}_{c} / T^{k,corp}_{c}$ & $R$-sample & $ICT$-sample \\\midrule
AT          &          44&           8&       19.18&          N/A&          N/A\\
BE          &          81&          15&       18.03&       39.61&       39.61\\
CZ          &         385&         179&       46.40&        0.16&        0.16\\
DE          &         410&          62&       15.23&          N/A&          N/A\\
DK          &         641&          60&        9.32&        7.62&        7.62\\
EE          &           2&           0&       21.88&        4.37&        4.12\\
ES          &         133&          25&       18.97&       35.34&       35.34\\
FI          &          36&           5&       13.33&       30.52&       30.52\\
FR          &         331&          45&       13.70&       19.10&       19.10\\
GR          &          21&           4&       20.43&        3.16&        3.16\\
HU          &       3,076&         831&       27.02&        0.10&          N/A\\
IE          &          31&           7&       23.56&        1.06&          N/A\\
IT          &         275&          36&       13.19&       27.11&       27.11\\
LT          &           2&           1&       27.26&        3.90&          N/A\\
LV          &           2&           0&       18.61&          N/A&          N/A\\
NL          &          85&          24&       27.96&        7.32&        7.32\\
PL          &         150&          34&       22.81&        6.84&          N/A\\
PT          &          21&           6&       27.49&       35.85&          N/A\\
SE          &         744&         121&       16.20&        1.36&        1.36\\
SI          &           3&           1&       21.35&        1.31&          N/A\\
SK          &           6&           3&       46.77&       31.92&       31.92\\
UK          &         311&          53&       17.12&       56.61&       56.61\\\midrule
Mean        &         309&          69&       22.08&       16.49&       20.30\\

         \bottomrule
        \end{tabular}
        \end{adjustbox}
        }\\
       \scriptsize
         Notes: Column (1) shows the total tax on capital $T^{k}$ in billions of national currency for each country in the last sample period, i.e. 2016. Column (2) is a sub-category of column (1) capturing corporate taxes on income, profits and capital gains $T^{k,corp}$ (with variable code 1200 in \citet{OECD2019} data set). Column (3) is the ratio of (1) over (2) in \%. Columns (4) and (5) capture the share of total taxes reported in the $R$- and $ICT$-sample used in the analysis, respectively, over (2) in \%. $R$- and $ICT$-sample refer to the firm level ORBIS sample when robot- and ICT-density is reported, respectively. The aggregate taxes cover the whole economy while the firm level samples cover the 15 industry-groupings discussed in detail in Appendix Table~\ref{tab:industry_codes}.  
    \end{table}

			    \begin{table}[H]
		            \caption{Summary statistics for firm level sample}
\label{tab:descriptives_firm}

	    \scriptsize
        {\centering
        \begin{adjustbox}{width=1\textwidth}
\begin{tabular}{lcccc}
\toprule
\csname @@input\endcsname{inputs/descriptives/Sumstat_firm}
\midrule
\csname @@input\endcsname{inputs/descriptives/Sumstat_firm_more}
\end{tabular}
\end{adjustbox}
}\\
\scriptsize
 Notes: $\dagger$ refers to values in thousands for the Mean, St.Dev., Min, Median, and Max. This table presents the summary statistics on the firm level corporate income tax ($T_{f,i,t}$) and number of employees ($L_{f,i,t}$) for 2 different samples. $R$- and $ICT$-sample refer to samples with non-missing values of industry level robot- and ICT-intensity, respectively. The $ICT$-sample covers the following 18 countries: AT; BE; CZ; DE; DK; EE; ES; FI; FR; GR; IT; LT; LV; NL; SE; SI; SK; and UK, while the $R$-sample covers 6 additional countries: HR; HU; IE; PL; PT; and RO. Both samples cover the same set of 15 industry groups included in the industry level analysis---for more details see Appendix Table~\ref{tab:industry_codes}.
\end{table}

\subsubsection{Additional results}
\label{appendix:add_results_local_effects}

\begin{figure}[H]
    {\centering
    \begin{subfigure}[r]{0.49\textwidth}
    
     \includegraphics[width=\linewidth]{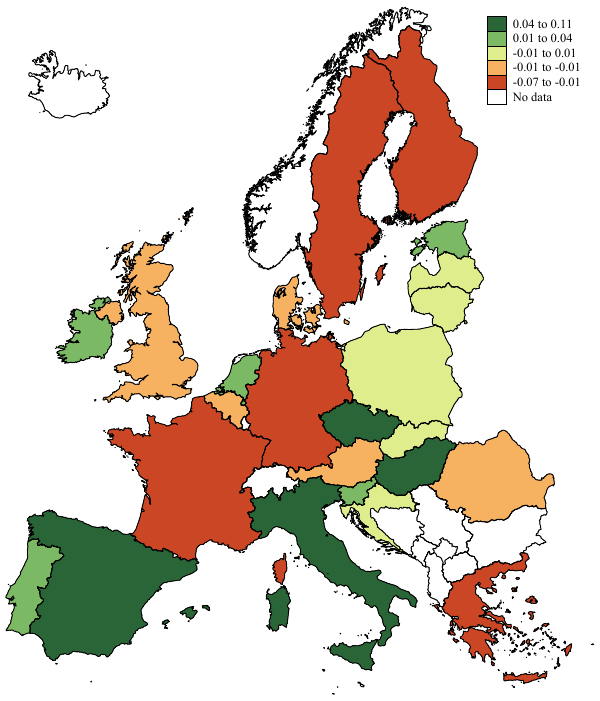}
     
     \subcaption{Labor \& robots}
    \end{subfigure}
        \begin{subfigure}[r]{0.49\textwidth}
     \includegraphics[width=\linewidth]{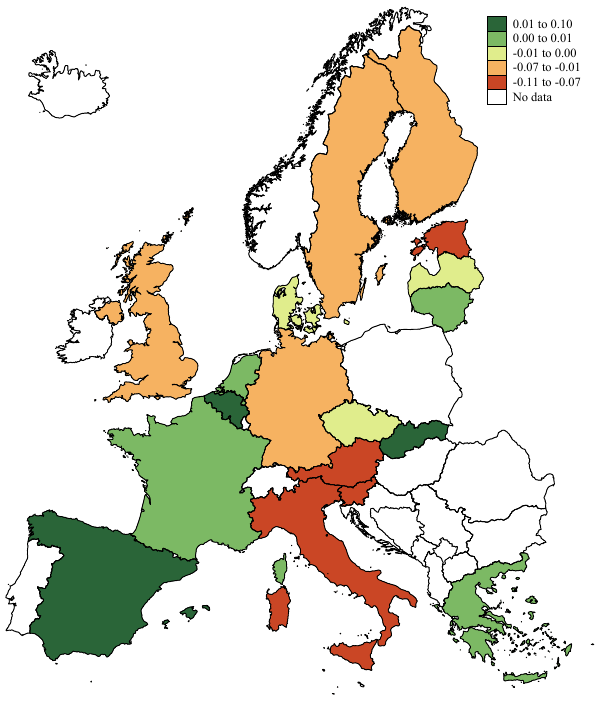}
     
        \subcaption{Labor \& ICT}
    \end{subfigure}
    
    \begin{subfigure}[r]{0.49\textwidth}
     \includegraphics[width=\linewidth]{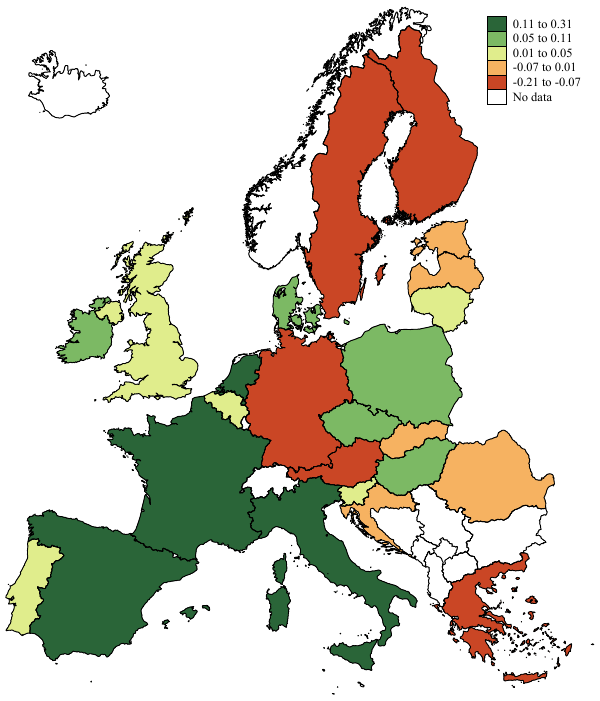}
     
    \subcaption{Taxes \& robots}
    \end{subfigure}
    \begin{subfigure}[r]{0.49\textwidth}
     \includegraphics[width=\linewidth]{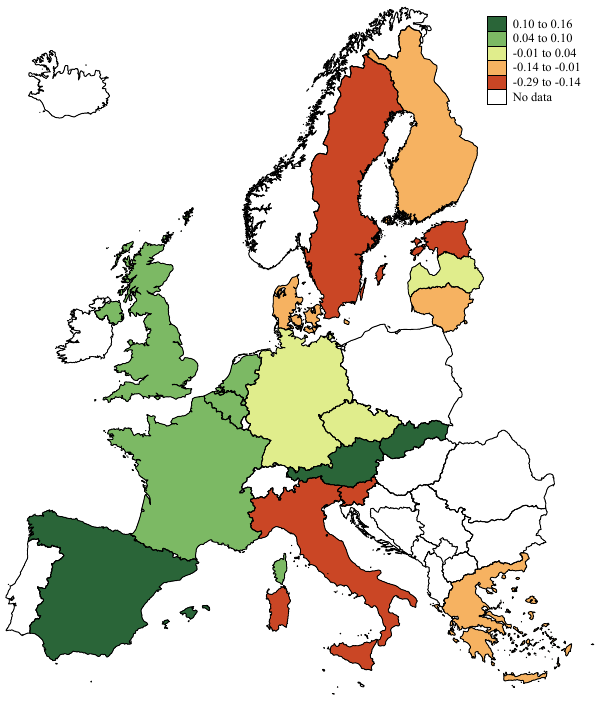}
     
    \subcaption{Taxes \& ICT}
    \end{subfigure}
    \caption{automation at the national level (NUTS0 regions)}
    \label{fig:ai_nuts0}
    }
    \scriptsize
    Source: Author's calculations based on ORBIS Global, IFR and EUKLEMS data sets.\\
    Notes: Each map presents the point estimates from regressing for each country separately the ln of the firm level corporate income tax ($Taxes$) and number of employees ($L$), respectively, on the industry level robot ($R$) or $ICT$ intensity. All regressions include firm and NUTS3 version 2016-region-year fixed effects and are weighted using the same weights as in the industry level analysis, i.e. base-sample-year share of each industry’s number of hours worked to country-wide hours worked. The estimated effects are plotted with 2 shades of green and red for two groups of positive and negative values, respectively, with the darker colors representing stronger effects. Regions with no data are left blank.    
\end{figure}

%\begin{comment}

\begin{figure}
    {\centering
    \begin{subfigure}[r]{0.49\textwidth}
    
     \includegraphics[width=\linewidth]{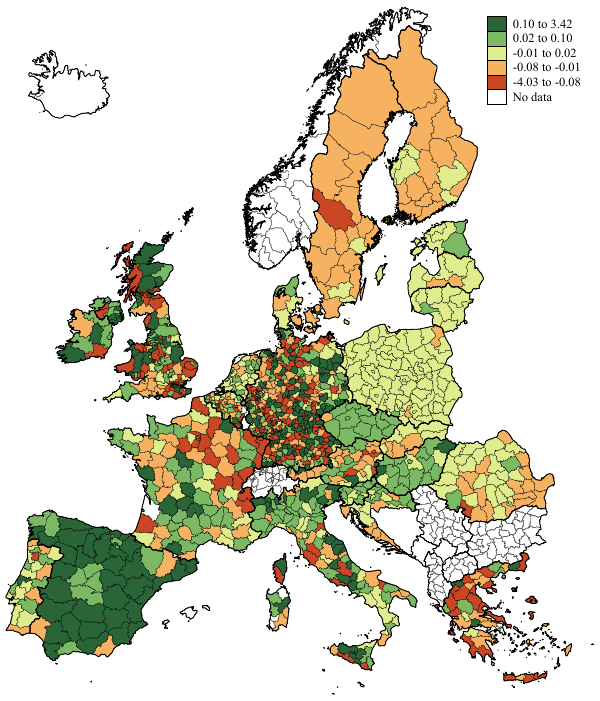}
     
     \subcaption{Labor \& robots}
    \end{subfigure}
        \begin{subfigure}[r]{0.49\textwidth}
     \includegraphics[width=\linewidth]{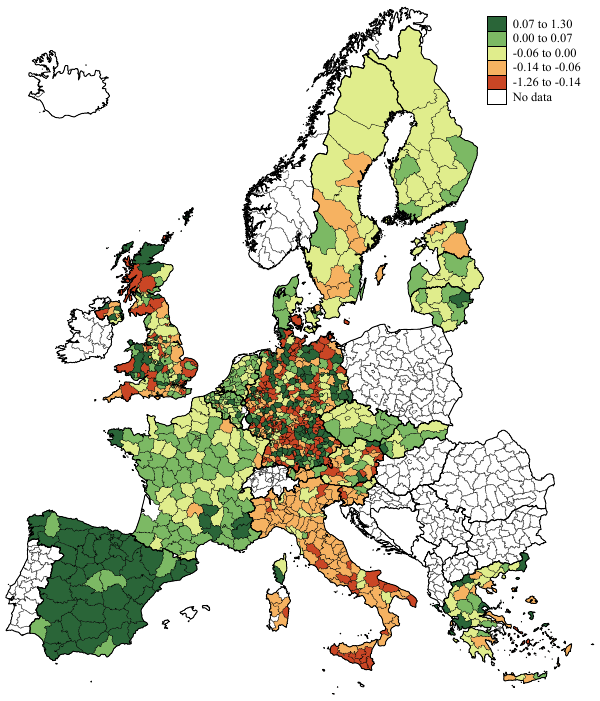}
     
        \subcaption{Labor \& ICT}
    \end{subfigure}
    
    \begin{subfigure}[r]{0.49\textwidth}
     \includegraphics[width=\linewidth]{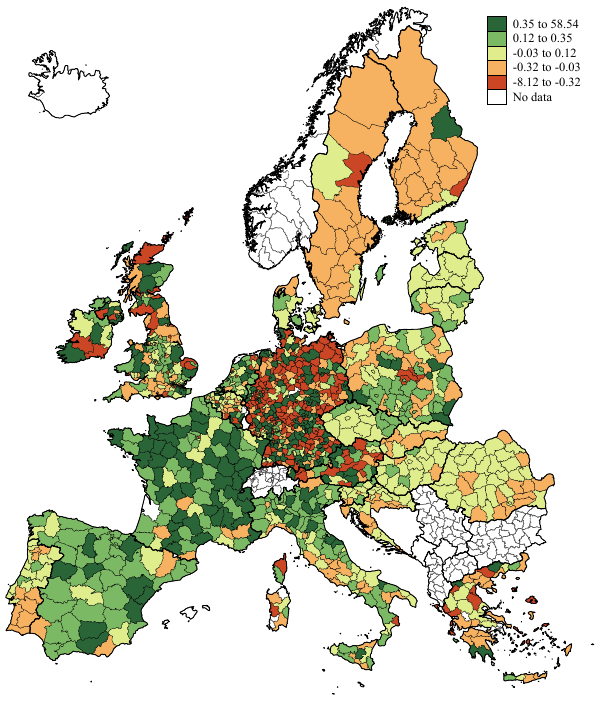}
     
    \subcaption{Taxes \& robots}
    \end{subfigure}
    \begin{subfigure}[r]{0.49\textwidth}
     \includegraphics[width=\linewidth]{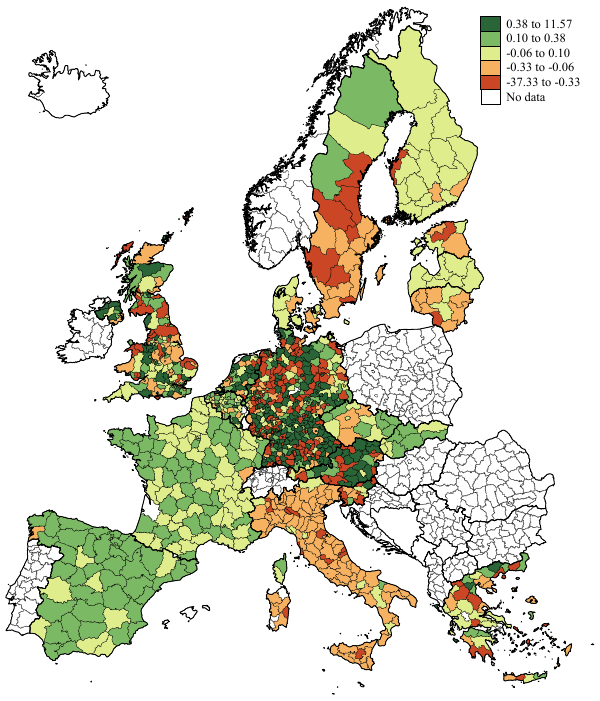}
     
    \subcaption{Taxes \& ICT}
    \end{subfigure}
    \caption{automation at the sub-national level (NUTS3 regions)}
    \label{fig:ai_nuts3}
    }
    \scriptsize
    Source: Author's calculations based on ORBIS Global, IFR and EUKLEMS data sets.\\
    Notes: Each map presents the point estimates from regressing for each country separately the ln of the firm level corporate income tax ($Taxes$) and number of employees ($L$), respectively, on the industry level robot ($R$) or $ICT$ intensity interacted with a full set of NUTS3 version 2016-regional dummies. All regressions include firm and NUTS3 version 2016-region-year fixed effects and are weighted using the same weights as in the industry level analysis, i.e. base-sample-year share of each industry’s number of hours worked to country-wide hours worked. The estimated effects are plotted with 2 shades of green and red for two groups of positive and negative values, respectively, with the darker colors representing stronger effects. Regions with no data are left blank. Panels (a), (b), (c) and (d) cover 1310, 1119, 1314, and 1123 NUTS3 regions, respectively.
\end{figure}
    
%\end{comment}

\FloatBarrier
\newpage
\section{Robustness: Coping with endogenous automation}
\label{SM:diffusion_endogeneity}
As explained in Sec. \ref{sec:empirical_approach_ai_data}, one major concern to the robustness of our results arises from potential endogeneity of AT diffusion. 
Ideally, we would like to measure the pure impact of technological progress in ATs as exogenous driver of AT diffusion to see how technological change affects the economy and public revenues. But we can only observe patterns of AT adoption which can endogenously dependent on economic dynamics. 

To cope with these concerns, we use three different types of robustness checks relying on lagged data and IVs. Here, we present the results of these robustness checks. 

In Sec. \ref{SM:robustness_lagged_controls}, we used robot- and ICT-intensity from $t-1$ instead of contemporaneous diffusion measures as explanatory variable. 
In Sec. \ref{SM:lagged_iv}, we used an IV approach. In particular, deeper lags from $t-1$, $t-2$ and $t-3$ are used as explanatory variables on the first stage to instrument contemporaneous AT diffusion. Below the tables with the results, we report statistics to test for under-, weak- and over-identification of the IV approach. The estimates of the coefficients of this approach are consistent with the results presented in the main text. 

Another IV approach is shown in Sec. \ref{SM:robustness_IV}. Here, we used robot and ICT products imports by all countries in the world except $c$ as in instrument for robot and ICT diffusion in country $c$.  This approach is inspired by \citet{blanas2019afraid} and follows the idea that AT imports to other countries should be driven by technological advances in ATs, but are entirely exogenous from the economic dynamics in country $c$. 
Again, we obtain qualitatively consistent point estimates for the coefficients, but the validity tests indicate a weak explanatory power at the first stage. 

Summing up, the lag-based and both IV approaches to cope with the endogeneity of AT diffusion measures support our analysis qualitatively, but the trade-based IV approach suffers from the weakness of instruments.\footnote{We have also experimented with alternative external IV approaches to construct Bartik-style instruments, but we ran into similar issues in terms of the validity of our instruments.}

\subsection{Using lagged ($t-1$) measures of ATs as controls}
\label{SM:robustness_lagged_controls}
\FloatBarrier
\subsubsection{Taxation and automation}

    \begin{table}[H]
    \caption{Taxation and automation}
    {\centering
    \begin{adjustbox}{width=\textwidth}\begin{tabular}{l|cccc|cccc|ccc}
    \toprule \addlinespace
\csname @@input\endcsname{inputs/robustness/lagged_controls/Results2shortV1_RICTint_ct_All_95t16}
\midrule
\csname @@input\endcsname{inputs/robustness/lagged_controls/Results2shortV1_RICTint_ct_All_95t07}
\midrule
\csname @@input\endcsname{inputs/robustness/lagged_controls/Results2shortV1_RICTint_ct_All_08t16}
\bottomrule
    \end{tabular}\end{adjustbox}} \\ 
    \label{tab:regr_pre_tax_robots_lagged_controls} \scriptsize
      Notes: $\ast$ \(p<0.05\), $\ast\ast$ \(p<0.01\), $\ast\ast\ast$ \(p<0.001\). Regression results of aggregate flows of tax revenues on different automation measures for 19 European countries during the period 2006-2016. All regressions use country level data and include: GDP growth, gross output share of the service sector in total economy; Herfindahl-Hirschman Index computed based on the gross-output shares of macro-sectors; government consolidated gross debt as \% of GDP; government interest payable as \% of GDP; net government lending/borrowing as \% of GDP; gross fixed capital formation as \% of GDP; period average exchange rate; effective tax rate; and country ($c$) and year ($t$) fixed effects. All regressions in Panel A also include the ln of gross-output value ($pQ$).
    \end{table}

\FloatBarrier
\newpage

\subsubsection{Taxation and economic production}

	\begin{table}[!ht]
	{\centering 
     
    \caption{Taxation and the structure of economic production for the period 2006-2016}
    \begin{adjustbox}{width=\textwidth}\begin{tabular}{l|cccc|cccc|ccc}
    
    \toprule \addlinespace
\csname @@input\endcsname{inputs/robustness/lagged_controls/Results2RICTint_ct_All_95t16}
\bottomrule
    \end{tabular}\end{adjustbox} \\ }

        \scriptsize
   Notes: $\ast$ \(p<0.05\), $\ast\ast$ \(p<0.01\), $\ast\ast\ast$ \(p<0.001\). Regression results to establish the link between tax aggregation and economic production for 19 European countries during the period 2006-2016. All regressions use country level data and include: GDP growth ($GDPgrowth_{c,t}$), share of gross output produced in service industries ($Services_{c,t}$); the Herfindahl-Hirschman Index computed based on the gross-output shares of macro-sectors ($HHI_{c,t}$); government consolidated gross debt as \% of GDP ($Debt^{\%GDP}_{c,t}$); government interest payable as \% of GDP ($Interest^{\%GDP}_{c,t}$); net government lending/borrowing as \% of GDP ($Lending^{\%GDP}_{c,t}$); gross fixed capital formation as \% of GDP ($GovInv^{\%GDP}_{c,t}$); period average exchange rate ($XRate_{c,t}$); effective tax rate ($ETR_{c,t}$); and country ($c$) and year ($t$) fixed effects. For the first block, $wL_{c,t}$, $rK_{c,t}$ and $pQ_{c,t}$ are expressed as the natural logarithm ($ln$) while for the last two blocks they are expressed as \% of GDP.
    \end{table}

	\subsubsection{The replacement effect}

			\begin{table}[H]
    {\centering 
    \caption{The replacement effect}
    \label{tab:regr_replacement_lag}
    \begin{adjustbox}{width=0.6\textwidth}\begin{tabular}{l|ccc|ccc}
    \toprule \addlinespace
    
    \csname @@input\endcsname{inputs/robustness/lagged_controls/Results3RICTint_cit_All_95t16}
    \bottomrule \addlinespace
\csname @@input\endcsname{inputs/robustness/lagged_controls/Results3RICTint_cit_All_95t07}
\bottomrule \addlinespace
\csname @@input\endcsname{inputs/robustness/lagged_controls/Results3RICTint_cit_All_08t16}
\bottomrule
    \end{tabular}\end{adjustbox}\\ }
    \scriptsize
    Notes: \sym{*}\(p<0.05\), \sym{**}\(p<0.01\), \sym{***}\(p<0.001\). Regression results to test the replacement effect for 19 European countries during the period 1995-2016. All regressions use industry level data for the subset of industries susceptible to automation, defined as industries were the use of industrial robots is prevalent (see Appendix Table~\ref{appendix:data}). All regressions include: country industry ($ci$); country year ($ct$); and industry year ($it$) fixed effects. All regressions are weighted by the base-sample-year share of each industry’s number of hours worked to country-wide hours worked. Standard errors are clustered both at the country-industry and year level.
    \end{table}

	\begin{table}[!ht]
	{\centering 
     
    \caption{Taxation and the structure of economic production for the period 1995-2007}
    \begin{adjustbox}{width=\textwidth}\begin{tabular}{l|cccc|cccc|ccc}
    
    \toprule \addlinespace

\csname @@input\endcsname{inputs/robustness/lagged_controls/Results2RICTint_ct_All_95t07}
\bottomrule
    \end{tabular}\end{adjustbox} \\ }

        \scriptsize
   Notes: $\ast$ \(p<0.05\), $\ast\ast$ \(p<0.01\), $\ast\ast\ast$ \(p<0.001\). Regression results to establish the link between tax aggregation and economic production for 19 European countries during the period 2006-2007. All regressions use country level data and include: GDP growth ($GDPgrowth_{c,t}$), share of gross output produced in service industries ($Services_{c,t}$); the Herfindahl-Hirschman Index computed based on the gross-output shares of macro-sectors ($HHI_{c,t}$); government consolidated gross debt as \% of GDP ($Debt^{\%GDP}_{c,t}$); government interest payable as \% of GDP ($Interest^{\%GDP}_{c,t}$); net government lending/borrowing as \% of GDP ($Lending^{\%GDP}_{c,t}$); gross fixed capital formation as \% of GDP ($GovInv^{\%GDP}_{c,t}$); period average exchange rate ($XRate_{c,t}$); effective tax rate ($ETR_{c,t}$); and country ($c$) and year ($t$) fixed effects. For the first block, $wL_{c,t}$, $rK_{c,t}$ and $pQ_{c,t}$ are expressed as the natural logarithm ($ln$) while for the last two blocks they are expressed as \% of GDP.
    \end{table}

	\begin{table}[!ht]
	{\centering 
     
    \caption{Taxation and the structure of economic production after 2008}
    \begin{adjustbox}{width=\textwidth}\begin{tabular}{l|cccc|cccc|ccc}
    
    \toprule \addlinespace
\csname @@input\endcsname{inputs/robustness/lagged_controls/Results2RICTint_ct_All_08t16}
\bottomrule
    \end{tabular}\end{adjustbox} \\ }

        \scriptsize
   Notes: $\ast$ \(p<0.05\), $\ast\ast$ \(p<0.01\), $\ast\ast\ast$ \(p<0.001\). Regression results to establish the link between tax aggregation and economic production for 19 European countries during the period 2008-2016. All regressions use country level data and include: GDP growth ($GDPgrowth_{c,t}$), share of gross output produced in service industries ($Services_{c,t}$); the Herfindahl-Hirschman Index computed based on the gross-output shares of macro-sectors ($HHI_{c,t}$); government consolidated gross debt as \% of GDP ($Debt^{\%GDP}_{c,t}$); government interest payable as \% of GDP ($Interest^{\%GDP}_{c,t}$); net government lending/borrowing as \% of GDP ($Lending^{\%GDP}_{c,t}$); gross fixed capital formation as \% of GDP ($GovInv^{\%GDP}_{c,t}$); period average exchange rate ($XRate_{c,t}$); effective tax rate ($ETR_{c,t}$); and country ($c$) and year ($t$) fixed effects. For the first block, $wL_{c,t}$, $rK_{c,t}$ and $pQ_{c,t}$ are expressed as the natural logarithm ($ln$) while for the last two blocks they are expressed as \% of GDP.
    \end{table}

\FloatBarrier	
\newpage
\subsubsection{The reinstatement effect}

		\begin{table}[!h]
    {\centering 
    \caption{The reinstatement effect}
    \label{tab:regr_reinstatement_lagged_controls_Eurostat}
    \begin{adjustbox}{width=0.9\textwidth}\begin{tabular}{l|cccccc}
    
    \toprule \addlinespace

\csname @@input\endcsname{inputs/robustness/lagged_controls/Results4shortRICTint_ct_All_95t16}
\bottomrule \addlinespace
\csname @@input\endcsname{inputs/robustness/lagged_controls/Results4shortRICTint_ct_All_95t07}
\bottomrule \addlinespace
\csname @@input\endcsname{inputs/robustness/lagged_controls/Results4shortRICTint_ct_All_08t16}
\bottomrule
    \end{tabular}\end{adjustbox}\\ }
    \scriptsize
    Notes: $\ast$ \(p<0.05\), $\ast\ast$ \(p<0.01\), $\ast\ast\ast$ \(p<0.001\). Regression results to test the reinstatement effect for 19 European countries during the period 2006-2016. All regressions include: GDP growth, government consolidated gross debt as \% of GDP; government interest payable as \% of GDP; net government lending/borrowing as \% of GDP; gross fixed capital formation as \% of GDP; period average exchange rate; value added TFP--calculated as the residual from an OLS regression of value-added volumes ($VA$) on a translog production function including capital volumes ($K$) and total number of hours worked ($L$); effective tax rate; and country ($c$) and year ($t$) fixed effects.
    \end{table}

\FloatBarrier
\newpage
\subsubsection{The real-income effect}

	\begin{table}[!h]
    {\centering 
        \caption{The real income effect}
            \label{tab:regr_realincome_lagged_controls_Eurostat}

    \begin{adjustbox}{width=\textwidth}\begin{tabular}{l|cccccccc}
    \toprule \addlinespace
\csname @@input\endcsname{inputs/robustness/lagged_controls/Results5RICTint_ct_All_95t16}
\bottomrule \addlinespace
\csname @@input\endcsname{inputs/robustness/lagged_controls/Results5RICTint_ct_All_95t07}
\bottomrule \addlinespace
\csname @@input\endcsname{inputs/robustness/lagged_controls/Results5RICTint_ct_All_08t16}
\bottomrule
    \end{tabular}\end{adjustbox}\\ \noindent }
    \scriptsize
    Notes: $\ast$ \(p<0.05\), $\ast\ast$ \(p<0.01\), $\ast\ast\ast$ \(p<0.001\). Regression results to test the real income effect for 19 European countries during the period 2006-2016. Labor productivity is measured as the share of gross-output volumes ($Q$) over the total number of hours worked. TFP is calculated as the residual from an OLS regression of gross-output volumes ($Q$) on a translog production function including capital volumes ($K$), total number of hours worked ($L$) and intermediate input volumes ($M$). All regressions include: GDP growth, government consolidated gross debt as \% of GDP; government interest payable as \% of GDP; net government lending/borrowing as \% of GDP; gross fixed capital formation as \% of GDP; period average exchange rate; effective tax rate; and country ($c$) and year ($t$) fixed effects.
    \end{table}

\FloatBarrier
\newpage

\subsection{Using deeper lags ($t-1$, $t-2$ , $t-3$) of AT measures as an IV}
\label{SM:lagged_iv}
\FloatBarrier
\subsubsection{Taxation and automation}

    \begin{table}[H]
    \caption{Taxation and automation}
    {\centering
    \begin{adjustbox}{width=\textwidth}\begin{tabular}{l|cccc|cccc|ccc}
    \toprule \addlinespace
\csname @@input\endcsname{inputs/robustness/IVlags/Results2shortV1_RICTint_ct_All_95t16}
\midrule
\csname @@input\endcsname{inputs/robustness/IVlags/Results2shortV1_RICTint_ct_All_95t07}
\midrule
\csname @@input\endcsname{inputs/robustness/IVlags/Results2shortV1_RICTint_ct_All_08t16}
\bottomrule
    \end{tabular}\end{adjustbox}} \\ 
    \label{tab:regr_pre_tax_robots_IVlags} \scriptsize
  Notes: $\ast$ \(p<0.05\), $\ast\ast$ \(p<0.01\), $\ast\ast\ast$ \(p<0.001\). Regression results of aggregate flows of tax revenues on different automation measures for 19 European countries during the period 2003-2016. All regressions use country level data and include: GDP growth, gross output share of the service sector in total economy; Herfindahl-Hirschman Index computed based on the gross-output shares of macro-sectors; government consolidated gross debt as \% of GDP; government interest payable as \% of GDP; net government lending/borrowing as \% of GDP; gross fixed capital formation as \% of GDP; period average exchange rate; corporate tax rate; and country ($c$) and year ($t$) fixed effects. All regressions in Panel A also include the ln of gross-output value ($pQ$).
    \end{table}

\FloatBarrier
\newpage
\subsubsection{Taxation and economic production}

	\begin{table}[!ht]
	{\centering 
     
    \caption{Taxation and the structure of economic production}
    \begin{adjustbox}{width=\textwidth}\begin{tabular}{l|cccc|cccc|ccc}
    
    \toprule \addlinespace
\csname @@input\endcsname{inputs/robustness/IVlags/Results2RICTint_ct_All_95t16}
\bottomrule
    \end{tabular}\end{adjustbox} \\ }

        \scriptsize
   Notes: $\ast$ \(p<0.05\), $\ast\ast$ \(p<0.01\), $\ast\ast\ast$ \(p<0.001\). Regression results to establish the link between tax aggregation and economic production for 19 European countries during the period 2003-2016. All regressions use country level data and include: GDP growth ($GDPgrowth_{c,t}$), share of gross output produced in service industries ($Services_{c,t}$); the Herfindahl-Hirschman Index computed based on the gross-output shares of macro-sectors ($HHI_{c,t}$); government consolidated gross debt as \% of GDP ($Debt^{\%GDP}_{c,t}$); government interest payable as \% of GDP ($Interest^{\%GDP}_{c,t}$); net government lending/borrowing as \% of GDP ($Lending^{\%GDP}_{c,t}$); gross fixed capital formation as \% of GDP ($GovInv^{\%GDP}_{c,t}$); period average exchange rate ($XRate_{c,t}$); corporate tax rate ($CTR_{c,t}$); and country ($c$) and year ($t$) fixed effects. For the first block, $wL_{c,t}$, $rK_{c,t}$ and $pQ_{c,t}$ are expressed as the natural logarithm ($ln$) while for the last two blocks they are expressed as \% of GDP.
    \end{table}

	\begin{table}[!ht]
	{\centering 
     
    \caption{Taxation and the structure of economic production for the period 2003-2007}
    \begin{adjustbox}{width=\textwidth}\begin{tabular}{l|cccc|cccc|ccc}
    
    \toprule \addlinespace

\csname @@input\endcsname{inputs/robustness/IVlags/Results2RICTint_ct_All_95t07}
\bottomrule
    \end{tabular}\end{adjustbox} \\ }

        \scriptsize
   Notes: $\ast$ \(p<0.05\), $\ast\ast$ \(p<0.01\), $\ast\ast\ast$ \(p<0.001\). Regression results to establish the link between tax aggregation and economic production for 19 European countries during the period 2003-2007. All regressions use country level data and include: GDP growth ($GDPgrowth_{c,t}$), share of gross output produced in service industries ($Services_{c,t}$); the Herfindahl-Hirschman Index computed based on the gross-output shares of macro-sectors ($HHI_{c,t}$); government consolidated gross debt as \% of GDP ($Debt^{\%GDP}_{c,t}$); government interest payable as \% of GDP ($Interest^{\%GDP}_{c,t}$); net government lending/borrowing as \% of GDP ($Lending^{\%GDP}_{c,t}$); gross fixed capital formation as \% of GDP ($GovInv^{\%GDP}_{c,t}$); period average exchange rate ($XRate_{c,t}$); corporate tax rate ($CTR_{c,t}$); and country ($c$) and year ($t$) fixed effects. For the first block, $wL_{c,t}$, $rK_{c,t}$ and $pQ_{c,t}$ are expressed as the natural logarithm ($ln$) while for the last two blocks they are expressed as \% of GDP.
    \end{table}

	\begin{table}[!ht]
	{\centering 
     
    \caption{Taxation and the structure of economic production after 2008}
    \begin{adjustbox}{width=\textwidth}\begin{tabular}{l|cccc|cccc|ccc}
    
    \toprule \addlinespace
\csname @@input\endcsname{inputs/robustness/IVlags/Results2RICTint_ct_All_08t16}
\bottomrule
    \end{tabular}\end{adjustbox} \\ }

        \scriptsize
   Notes: $\ast$ \(p<0.05\), $\ast\ast$ \(p<0.01\), $\ast\ast\ast$ \(p<0.001\). Regression results to establish the link between tax aggregation and economic production for 19 European countries during the period 2008-2016. All regressions use country level data and include: GDP growth ($GDPgrowth_{c,t}$), share of gross output produced in service industries ($Services_{c,t}$); the Herfindahl-Hirschman Index computed based on the gross-output shares of macro-sectors ($HHI_{c,t}$); government consolidated gross debt as \% of GDP ($Debt^{\%GDP}_{c,t}$); government interest payable as \% of GDP ($Interest^{\%GDP}_{c,t}$); net government lending/borrowing as \% of GDP ($Lending^{\%GDP}_{c,t}$); gross fixed capital formation as \% of GDP ($GovInv^{\%GDP}_{c,t}$); period average exchange rate ($XRate_{c,t}$); corporate tax rate ($CTR_{c,t}$); and country ($c$) and year ($t$) fixed effects. For the first block, $wL_{c,t}$, $rK_{c,t}$ and $pQ_{c,t}$ are expressed as the natural logarithm ($ln$) while for the last two blocks they are expressed as \% of GDP.
    \end{table}

\FloatBarrier	
\newpage
\subsubsection{The replacement effect}

			\begin{table}[H]
    {\centering 
    \caption{The replacement effect}
    \label{tab:regr_replacement_ivlag}
    \begin{adjustbox}{width=0.6\textwidth}\begin{tabular}{l|ccc|ccc}
    \toprule \addlinespace
    
    \csname @@input\endcsname{inputs/robustness/IVlags/Results3RICTint_cit_All_95t16}
    \bottomrule \addlinespace
\csname @@input\endcsname{inputs/robustness/IVlags/Results3RICTint_cit_All_95t07}
\bottomrule \addlinespace
\csname @@input\endcsname{inputs/robustness/IVlags/Results3RICTint_cit_All_08t16}
\bottomrule
    \end{tabular}\end{adjustbox}\\ }
    \scriptsize
    Notes: \sym{*}\(p<0.05\), \sym{**}\(p<0.01\), \sym{***}\(p<0.001\). Regression results to test the replacement effect for 19 European countries during the period 1995-2016. All regressions use industry level data for the subset of industries susceptible to automation, defined as industries were the use of industrial robots is prevalent (see Appendix Table~\ref{appendix:data}). All regressions include: country industry ($ci$); country year ($ct$); and industry year ($it$) fixed effects. All regressions are weighted by the base-sample-year share of each industry’s number of hours worked to country-wide hours worked. Standard errors are clustered both at the country-industry and year level.
    \end{table}

\subsubsection{The reinstatement effect}

		\begin{table}[!h]
    {\centering 
    \caption{The reinstatement effect}
    \label{tab:regr_reinstatement_IVlags}
    \begin{adjustbox}{width=0.9\textwidth}\begin{tabular}{l|cccccc}
    
    \toprule \addlinespace
\csname @@input\endcsname{inputs/robustness/IVlags/Results4shortRICTint_ct_All_95t16}
\bottomrule \addlinespace
\csname @@input\endcsname{inputs/robustness/IVlags/Results4shortRICTint_ct_All_95t07}
\bottomrule \addlinespace
\csname @@input\endcsname{inputs/robustness/IVlags/Results4shortRICTint_ct_All_08t16}
\bottomrule
    \end{tabular}\end{adjustbox}\\ }
    \scriptsize
    Notes: $\ast$ \(p<0.05\), $\ast\ast$ \(p<0.01\), $\ast\ast\ast$ \(p<0.001\). Regression results to test the reinstatement effect for 19 European countries during the period 2003-2016. All regressions include: GDP growth, government consolidated gross debt as \% of GDP; government interest payable as \% of GDP; net government lending/borrowing as \% of GDP; gross fixed capital formation as \% of GDP; period average exchange rate; value added TFP--calculated as the residual from an OLS regression of value-added volumes ($VA$) on a translog production function including capital volumes ($K$) and total number of hours worked ($L$); corporate tax rate; and country ($c$) and year ($t$) fixed effects.
    \end{table}

\FloatBarrier
\newpage
\subsubsection{The real-income effect}

	\begin{table}[!h]
    {\centering 
        \caption{The real income effect}
            \label{tab:regr_realincome_IVlags}

    \begin{adjustbox}{width=0.9\textwidth}\begin{tabular}{l|cccccccc}
    \toprule \addlinespace
\csname @@input\endcsname{inputs/robustness/IVlags/Results5RICTint_ct_All_95t16}
\bottomrule \addlinespace
\csname @@input\endcsname{inputs/robustness/IVlags/Results5RICTint_ct_All_95t07}
\bottomrule \addlinespace
\csname @@input\endcsname{inputs/robustness/IVlags/Results5RICTint_ct_All_08t16}
\bottomrule
    \end{tabular}\end{adjustbox}\\ \noindent }
    \scriptsize
    Notes: $\ast$ \(p<0.05\), $\ast\ast$ \(p<0.01\), $\ast\ast\ast$ \(p<0.001\). Regression results to test the real income effect for 19 European countries during the period 2003-2016. Labor productivity is measured as the share of gross-output volumes ($Q$) over the total number of hours worked. TFP is calculated as the residual from an OLS regression of gross-output volumes ($Q$) on a translog production function including capital volumes ($K$), total number of hours worked ($L$) and intermediate input volumes ($M$). All regressions include: GDP growth, government consolidated gross debt as \% of GDP; government interest payable as \% of GDP; net government lending/borrowing as \% of GDP; gross fixed capital formation as \% of GDP; period average exchange rate; corporate tax rate; and country ($c$) and year ($t$) fixed effects.
    \end{table}

\FloatBarrier
%\newpage

\subsection{Using trade data on imports of robot and ICT products to construct external IVs for the AT measures}

%\clearpage
\label{SM:robustness_IV}
\FloatBarrier
\subsubsection{Taxation and automation}

    \begin{table}[H]
    \caption{Taxation and automation}
    {\centering
    \begin{adjustbox}{width=0.9\textwidth}\begin{tabular}{l|cccc|cccc|ccc}
    \toprule \addlinespace
\csname @@input\endcsname{inputs/robustness/IV/Results2shortV1_RICTint_ct_All_95t16}
\midrule
\csname @@input\endcsname{inputs/robustness/IV/Results2shortV1_RICTint_ct_All_95t07}
\midrule
\csname @@input\endcsname{inputs/robustness/IV/Results2shortV1_RICTint_ct_All_08t16}
\bottomrule
    \end{tabular}\end{adjustbox} \\ }
    \label{tab:regr_pre_tax_robots_IV} \scriptsize
  Notes: $\ast$ \(p<0.05\), $\ast\ast$ \(p<0.01\), $\ast\ast\ast$ \(p<0.001\). Regression results of aggregate flows of tax revenues on different automation measures for 19 European countries during the period 1995-2016. All regressions use country level data and include: GDP growth, gross output share of the service sector in total economy; Herfindahl-Hirschman Index computed based on the gross-output shares of macro-sectors; government consolidated gross debt as \% of GDP; government interest payable as \% of GDP; net government lending/borrowing as \% of GDP; gross fixed capital formation as \% of GDP; period average exchange rate; imports as \% of GDP; exports as \% of GDP; and country ($c$) and year ($t$) fixed effects. All regressions in Panel A also include the ln of gross-output value ($pQ$).
    \end{table}

\FloatBarrier
\newpage
\subsubsection{Taxation and economic production}

	\begin{table}[!ht]
	{\centering 
     
    \caption{Taxation and the structure of economic production}
    \begin{adjustbox}{width=\textwidth}\begin{tabular}{l|cccc|cccc|ccc}
    
    \toprule \addlinespace
\csname @@input\endcsname{inputs/robustness/IV/Results2RICTint_ct_All_95t16}
\bottomrule
    \end{tabular}\end{adjustbox} \\ }

        \scriptsize
   Notes: $\ast$ \(p<0.05\), $\ast\ast$ \(p<0.01\), $\ast\ast\ast$ \(p<0.001\). Regression results to establish the link between tax aggregation and economic production for 19 European countries during the period 1995-2016. All regressions use country level data and include: GDP growth ($GDPgrowth_{c,t}$), share of gross output produced in service industries ($Services_{c,t}$); the Herfindahl-Hirschman Index computed based on the gross-output shares of macro-sectors ($HHI_{c,t}$); government consolidated gross debt as \% of GDP ($Debt^{\%GDP}_{c,t}$); government interest payable as \% of GDP ($Interest^{\%GDP}_{c,t}$); net government lending/borrowing as \% of GDP ($Lending^{\%GDP}_{c,t}$); gross fixed capital formation as \% of GDP ($GovInv^{\%GDP}_{c,t}$); period average exchange rate ($XRate_{c,t}$); imports as \% of GDP ($Imports^{\%GDP}_{c,t}$); exports as \% of GDP ($Exports^{\%GDP}_{c,t}$); and country ($c$) and year ($t$) fixed effects. For the first block, $wL_{c,t}$, $rK_{c,t}$ and $pQ_{c,t}$ are expressed as the natural logarithm ($ln$) while for the last two blocks they are expressed as \% of GDP.
    \end{table}

	\begin{table}[!ht]
	{\centering 
     
    \caption{Taxation and the structure of economic production before 2007}
    \begin{adjustbox}{width=\textwidth}\begin{tabular}{l|cccc|cccc|ccc}
    
    \toprule \addlinespace

\csname @@input\endcsname{inputs/robustness/IV/Results2RICTint_ct_All_95t07}
\bottomrule
    \end{tabular}\end{adjustbox} \\ }

        \scriptsize
   Notes: $\ast$ \(p<0.05\), $\ast\ast$ \(p<0.01\), $\ast\ast\ast$ \(p<0.001\). Regression results to establish the link between tax aggregation and economic production for 19 European countries during the period 1995-2007. All regressions use country level data and include: GDP growth ($GDPgrowth_{c,t}$), share of gross output produced in service industries ($Services_{c,t}$); the Herfindahl-Hirschman Index computed based on the gross-output shares of macro-sectors ($HHI_{c,t}$); government consolidated gross debt as \% of GDP ($Debt^{\%GDP}_{c,t}$); government interest payable as \% of GDP ($Interest^{\%GDP}_{c,t}$); net government lending/borrowing as \% of GDP ($Lending^{\%GDP}_{c,t}$); gross fixed capital formation as \% of GDP ($GovInv^{\%GDP}_{c,t}$); period average exchange rate ($XRate_{c,t}$); imports as \% of GDP ($Imports^{\%GDP}_{c,t}$); exports as \% of GDP ($Exports^{\%GDP}_{c,t}$); and country ($c$) and year ($t$) fixed effects. For the first block, $wL_{c,t}$, $rK_{c,t}$ and $pQ_{c,t}$ are expressed as the natural logarithm ($ln$) while for the last two blocks they are expressed as \% of GDP.
    \end{table}

	\begin{table}[!ht]
	{\centering 
     
    \caption{Taxation and the structure of economic production after 2008}
    \begin{adjustbox}{width=\textwidth}\begin{tabular}{l|cccc|cccc|ccc}
    
    \toprule \addlinespace
\csname @@input\endcsname{inputs/robustness/IV/Results2RICTint_ct_All_08t16}
\bottomrule
    \end{tabular}\end{adjustbox} \\ }

        \scriptsize
   Notes: $\ast$ \(p<0.05\), $\ast\ast$ \(p<0.01\), $\ast\ast\ast$ \(p<0.001\). Regression results to establish the link between tax aggregation and economic production for 19 European countries during the period 2008-2016. All regressions use country level data and include: GDP growth ($GDPgrowth_{c,t}$), share of gross output produced in service industries ($Services_{c,t}$); the Herfindahl-Hirschman Index computed based on the gross-output shares of macro-sectors ($HHI_{c,t}$); government consolidated gross debt as \% of GDP ($Debt^{\%GDP}_{c,t}$); government interest payable as \% of GDP ($Interest^{\%GDP}_{c,t}$); net government lending/borrowing as \% of GDP ($Lending^{\%GDP}_{c,t}$); gross fixed capital formation as \% of GDP ($GovInv^{\%GDP}_{c,t}$); period average exchange rate ($XRate_{c,t}$); imports as \% of GDP ($Imports^{\%GDP}_{c,t}$); exports as \% of GDP ($Exports^{\%GDP}_{c,t}$); and country ($c$) and year ($t$) fixed effects. For the first block, $wL_{c,t}$, $rK_{c,t}$ and $pQ_{c,t}$ are expressed as the natural logarithm ($ln$) while for the last two blocks they are expressed as \% of GDP.
    \end{table}

\FloatBarrier	
\newpage
\subsubsection{The reinstatement effect}

		\begin{table}[!h]
    {\centering 
    \caption{The reinstatement effect}
    \label{tab:regr_reinstatement_IV}
    \begin{adjustbox}{width=\textwidth,totalheight=0.80\textheight,keepaspectratio}\begin{tabular}{l|cccccc}
    
    \toprule \addlinespace

\csname @@input\endcsname{inputs/robustness/IV/Results4shortRICTint_ct_All_95t16}
\bottomrule \addlinespace
\csname @@input\endcsname{inputs/robustness/IV/Results4shortRICTint_ct_All_95t07}
\bottomrule \addlinespace
\csname @@input\endcsname{inputs/robustness/IV/Results4shortRICTint_ct_All_08t16}
\bottomrule
    \end{tabular}\end{adjustbox}\\ }
    \scriptsize
    Notes: $\ast$ \(p<0.05\), $\ast\ast$ \(p<0.01\), $\ast\ast\ast$ \(p<0.001\). Regression results to test the reinstatement effect for 19 European countries during the period 1995-2016. All regressions include: GDP growth, government consolidated gross debt as \% of GDP; government interest payable as \% of GDP; net government lending/borrowing as \% of GDP; gross fixed capital formation as \% of GDP; period average exchange rate; value added TFP--calculated as the residual from an OLS regression of value-added volumes ($VA$) on a translog production function including capital volumes ($K$) and total number of hours worked ($L$); imports as \% of GDP; exports as \% of GDP; and country ($c$) and year ($t$) fixed effects.
    \end{table}

\FloatBarrier
\newpage
\subsubsection{The real-income effect}

	\begin{table}[!h]
    {\centering 
        \caption{The real income effect}
            \label{tab:regr_realincome_IV}

    \begin{adjustbox}{width=0.90\textwidth}\begin{tabular}{l|cccccccc}
    \toprule \addlinespace
\csname @@input\endcsname{inputs/robustness/IV/Results5RICTint_ct_All_95t16}
\bottomrule \addlinespace
\csname @@input\endcsname{inputs/robustness/IV/Results5RICTint_ct_All_95t07}
\bottomrule \addlinespace
\csname @@input\endcsname{inputs/robustness/IV/Results5RICTint_ct_All_08t16}
\bottomrule
    \end{tabular}\end{adjustbox}\\ \noindent }
    \scriptsize
    Notes: $\ast$ \(p<0.05\), $\ast\ast$ \(p<0.01\), $\ast\ast\ast$ \(p<0.001\). Regression results to test the real income effect for 19 European countries during the period 1995-2016. Labor productivity is measured as the share of gross-output volumes ($Q$) over the total number of hours worked. TFP is calculated as the residual from an OLS regression of gross-output volumes ($Q$) on a translog production function including capital volumes ($K$), total number of hours worked ($L$) and intermediate input volumes ($M$). All regressions include: GDP growth, government consolidated gross debt as \% of GDP; government interest payable as \% of GDP; net government lending/borrowing as \% of GDP; gross fixed capital formation as \% of GDP; period average exchange rate; imports as \% of GDP; exports as \% of GDP; and country ($c$) and year ($t$) fixed effects.
    \end{table}

\FloatBarrier
\newpage
\FloatBarrier
\newpage
\section{Robustness checks: Taxes, trade and income distribution}
\label{SM:robustness_taxes}

In this section, we provide the results of a series of robustness checks. 

First, we make sure that our results are not driven by changes in the tax system. Unfortunately, comprehensive data that covers the whole range of different taxes, that is consistent across our sample of countries and covers a reasonable number of years is not available. 
We are only able to proxy tax reforms using data on corporate taxation that cover a smaller period of time but all countries in our sample. We use two different data sources. 

In \ref{SM:robustness_KPMG}, we repeat all baseline country level regressions and include as an additional control the corporate tax rate ($CRT_{c,t}$) sourced from KPMG.\footnote{The data were sourced from the KPMG website: \url{https://home.kpmg/xx/en/home/services/tax/tax-tools-and-resources/tax-rates-online.html}} 
This data are only available between 2003-2016 and only the results for the period after 2008 are comparable with the baseline analysis.

Next, in \ref{SM:robustness_ETR_Eurostat} we repeat all baseline country level regressions and include as an additional control the effective tax rate ($ERT_{c,t}$) sourced from Eurostat.\footnote{This is the Effective Average Tax Rate (ETR) for large corporations in non-financial sector, computed at corporate level, for average asset composition and funding sources, using the Devereux/Griffith 
 methodology. The data are available in Eurostat: \url{https://ec.europa.eu/taxation_customs/business/economic-analysis-taxation/data-taxation_en}} 
The ETR variable is only available between 2006-2016 and again, only the results for the period after 2008 are comparable with the baseline analysis.
 
Another concern regarding the robustness of our results may arise from the impact of trade. In our baseline, we only controlled for the exchange rate which does not or only poorly vary across different European countries. To capture the country specific impact of trade, we repeat all baseline country level regressions and include as additional controls the countrylevel imports ($Imports^{\% GDP}_{c,t}$) and exports ($Exports^{\% GDP}_{c,t}$) as percentage of GDP sourced from the OECD National Accounts Database.\footnote{The data are available in OECD: \url{https://stats.oecd.org/viewhtml.aspx?datasetcode=NAAG\&lang=en\#}} 
The results are shown in Table \ref{SM:robustness_trade}. 
%Note that, similar to the baseline analysis, the additional variables are available for all years, i.e. 1995-2016.

\begin{comment}
To support the interpretation of our results, we examine the relationship between automation and income distribution and between income distribution and taxation. 

In \ref{SM:robustness_distribution} illustrate the distributional effect of AT diffusion. We rely on the same empirical specification used to estimate the reinstatement effects, but now our regressions are based on the following four left hand side variables: two Gini coefficients from the industry level distribution of hourly wage ($Gini^{w}_{c,t}$) and labor in terms of hours worked ($Gini^{L}_{c,t}$), respectively; and two dispersion measures computed as the 90/10 percentile ratio from the industry level distribution of hourly wage ($Dispersion^{w}_{c,t}$) and labor in terms of hours worked ($Dispersion^{L}_{c,t}$), respectively. To construct the measures we use the EUKLEMS dataset.
\end{comment}
Further, to explore the nexus between distribution and taxation, we examine the progressiveness of taxation (Table \ref{SM:robustness_progressive}). To do so, we rely on the same empirical specification used to understand the determinants of taxation, but now our regressions include as an additional control the Gini coefficient from the industry level distribution of labor in terms of hours worked ($Gini^{L}_{c,t}$) sourced from Eurostat.

Finally, we also test whether the attribution of capital taxes within the broad categories from OECD might affect our results. In particular we test whether the exclusion of the OECD tax category 1100 ``taxes on income, profits and capital gains of individuals'' from the taxes on capital $T^k$ changes the interpretation of our findings (assuming that these are neither capital nor labor taxes in the strict sense of their origin). The results are presented in \ref{SM:robustness_Tk} where we find similar results as in our baseline but the share of taxes as a percent of total taxes and GDP drops significantly due to this omission.

\subsection{Controlling for changes in corporate taxation using KPMG data}
\label{SM:robustness_KPMG}
\FloatBarrier
\subsubsection{Taxation and automation}

    \begin{table}[H]
    \caption{Taxation and automation}
    {
    \begin{adjustbox}{width=0.85\textwidth}
    \centering
    \begin{tabular}{l|cccc|cccc|ccc}
    \toprule \addlinespace
\csname @@input\endcsname{inputs/robustness/CTR_KPMG/Results2shortV1_RICTint_ct_All_95t16}
\midrule
\csname @@input\endcsname{inputs/robustness/CTR_KPMG/Results2shortV1_RICTint_ct_All_95t07}
\midrule
\csname @@input\endcsname{inputs/robustness/CTR_KPMG/Results2shortV1_RICTint_ct_All_08t16}
\bottomrule
    \end{tabular}\end{adjustbox}} \\ 
    \label{tab:regr_pre_tax_robots_KPMG} \scriptsize
  Notes: $\ast$ \(p<0.05\), $\ast\ast$ \(p<0.01\), $\ast\ast\ast$ \(p<0.001\). Regression results of aggregate flows of tax revenues on different automation measures for 19 European countries during the period 2003-2016. All regressions use country level data and include: GDP growth, gross output share of the service sector in total economy; Herfindahl-Hirschman Index computed based on the gross-output shares of macro-sectors; government consolidated gross debt as \% of GDP; government interest payable as \% of GDP; net government lending/borrowing as \% of GDP; gross fixed capital formation as \% of GDP; period average exchange rate; corporate tax rate; and country ($c$) and year ($t$) fixed effects. All regressions in Panel A also include the ln of gross-output value ($pQ$).
    \end{table}

\FloatBarrier
\newpage
\subsubsection{Taxation and economic production}

	\begin{table}[!ht]
	{\centering 
     
    \caption{Taxation and the structure of economic production for the period 2003-2016}
    \begin{adjustbox}{width=\textwidth}\begin{tabular}{l|cccc|cccc|ccc}
    
    \toprule \addlinespace
\csname @@input\endcsname{inputs/robustness/CTR_KPMG/Results2RICTint_ct_All_95t16}
\bottomrule
    \end{tabular}\end{adjustbox} \\ }

        \scriptsize
   Notes: $\ast$ \(p<0.05\), $\ast\ast$ \(p<0.01\), $\ast\ast\ast$ \(p<0.001\). Regression results to establish the link between tax aggregation and economic production for 19 European countries during the period 2003-2016. All regressions use country level data and include: GDP growth ($GDPgrowth_{c,t}$), share of gross output produced in service industries ($Services_{c,t}$); the Herfindahl-Hirschman Index computed based on the gross-output shares of macro-sectors ($HHI_{c,t}$); government consolidated gross debt as \% of GDP ($Debt^{\%GDP}_{c,t}$); government interest payable as \% of GDP ($Interest^{\%GDP}_{c,t}$); net government lending/borrowing as \% of GDP ($Lending^{\%GDP}_{c,t}$); gross fixed capital formation as \% of GDP ($GovInv^{\%GDP}_{c,t}$); period average exchange rate ($XRate_{c,t}$); corporate tax rate ($CTR_{c,t}$); and country ($c$) and year ($t$) fixed effects. For the first block, $wL_{c,t}$, $rK_{c,t}$ and $pQ_{c,t}$ are expressed as the natural logarithm ($ln$) while for the last two blocks they are expressed as \% of GDP.
    \end{table}

	\begin{table}[!ht]
	{\centering 
     
    \caption{Taxation and the structure of economic production for the period 2003-2007}
    \begin{adjustbox}{width=\textwidth}\begin{tabular}{l|cccc|cccc|ccc}
    
    \toprule \addlinespace

\csname @@input\endcsname{inputs/robustness/CTR_KPMG/Results2RICTint_ct_All_95t07}
\bottomrule
    \end{tabular}\end{adjustbox} \\ }

        \scriptsize
   Notes: $\ast$ \(p<0.05\), $\ast\ast$ \(p<0.01\), $\ast\ast\ast$ \(p<0.001\). Regression results to establish the link between tax aggregation and economic production for 19 European countries during the period 2003-2007. All regressions use country level data and include: GDP growth ($GDPgrowth_{c,t}$), share of gross output produced in service industries ($Services_{c,t}$); the Herfindahl-Hirschman Index computed based on the gross-output shares of macro-sectors ($HHI_{c,t}$); government consolidated gross debt as \% of GDP ($Debt^{\%GDP}_{c,t}$); government interest payable as \% of GDP ($Interest^{\%GDP}_{c,t}$); net government lending/borrowing as \% of GDP ($Lending^{\%GDP}_{c,t}$); gross fixed capital formation as \% of GDP ($GovInv^{\%GDP}_{c,t}$); period average exchange rate ($XRate_{c,t}$); corporate tax rate ($CTR_{c,t}$); and country ($c$) and year ($t$) fixed effects. For the first block, $wL_{c,t}$, $rK_{c,t}$ and $pQ_{c,t}$ are expressed as the natural logarithm ($ln$) while for the last two blocks they are expressed as \% of GDP.
    \end{table}

	\begin{table}[!ht]
	{\centering 
     
    \caption{Taxation and the structure of economic production after 2008}
    \begin{adjustbox}{width=\textwidth}\begin{tabular}{l|cccc|cccc|ccc}
    
    \toprule \addlinespace
\csname @@input\endcsname{inputs/robustness/CTR_KPMG/Results2RICTint_ct_All_08t16}
\bottomrule
    \end{tabular}\end{adjustbox} \\ }

        \scriptsize
   Notes: $\ast$ \(p<0.05\), $\ast\ast$ \(p<0.01\), $\ast\ast\ast$ \(p<0.001\). Regression results to establish the link between tax aggregation and economic production for 19 European countries during the period 2008-2016. All regressions use country level data and include: GDP growth ($GDPgrowth_{c,t}$), share of gross output produced in service industries ($Services_{c,t}$); the Herfindahl-Hirschman Index computed based on the gross-output shares of macro-sectors ($HHI_{c,t}$); government consolidated gross debt as \% of GDP ($Debt^{\%GDP}_{c,t}$); government interest payable as \% of GDP ($Interest^{\%GDP}_{c,t}$); net government lending/borrowing as \% of GDP ($Lending^{\%GDP}_{c,t}$); gross fixed capital formation as \% of GDP ($GovInv^{\%GDP}_{c,t}$); period average exchange rate ($XRate_{c,t}$); corporate tax rate ($CTR_{c,t}$); and country ($c$) and year ($t$) fixed effects. For the first block, $wL_{c,t}$, $rK_{c,t}$ and $pQ_{c,t}$ are expressed as the natural logarithm ($ln$) while for the last two blocks they are expressed as \% of GDP.
    \end{table}

\FloatBarrier	
\newpage

\subsubsection{The reinstatement effect}

		\begin{table}[!h]
    {\centering 
    \caption{The reinstatement effect}
    \label{tab:regr_reinstatement_KPMG}
    \begin{adjustbox}{width=0.9\textwidth}\begin{tabular}{l|cccccc}
    
    \toprule \addlinespace
\csname @@input\endcsname{inputs/robustness/CTR_KPMG/Results4shortRICTint_ct_All_95t16}
\bottomrule \addlinespace
\csname @@input\endcsname{inputs/robustness/CTR_KPMG/Results4shortRICTint_ct_All_95t07}
\bottomrule \addlinespace
\csname @@input\endcsname{inputs/robustness/CTR_KPMG/Results4shortRICTint_ct_All_08t16}
\bottomrule
    \end{tabular}\end{adjustbox}\\ }
    \scriptsize
    Notes: $\ast$ \(p<0.05\), $\ast\ast$ \(p<0.01\), $\ast\ast\ast$ \(p<0.001\). Regression results to test the reinstatement effect for 19 European countries during the period 2003-2016. All regressions include: GDP growth, government consolidated gross debt as \% of GDP; government interest payable as \% of GDP; net government lending/borrowing as \% of GDP; gross fixed capital formation as \% of GDP; period average exchange rate; value added TFP--calculated as the residual from an OLS regression of value-added volumes ($VA$) on a translog production function including capital volumes ($K$) and total number of hours worked ($L$); corporate tax rate; and country ($c$) and year ($t$) fixed effects.
    \end{table}

\FloatBarrier
\newpage
\subsubsection{The real-income effect}

	\begin{table}[!h]
    {\centering 
        \caption{The real income effect}
            \label{tab:regr_realincome_KPMG}

    \begin{adjustbox}{width=\textwidth}\begin{tabular}{l|cccccccc}
    \toprule \addlinespace
\csname @@input\endcsname{inputs/robustness/CTR_KPMG/Results5RICTint_ct_All_95t16}
\bottomrule \addlinespace
\csname @@input\endcsname{inputs/robustness/CTR_KPMG/Results5RICTint_ct_All_95t07}
\bottomrule \addlinespace
\csname @@input\endcsname{inputs/robustness/CTR_KPMG/Results5RICTint_ct_All_08t16}
\bottomrule
    \end{tabular}\end{adjustbox}\\ \noindent }
    \scriptsize
    Notes: $\ast$ \(p<0.05\), $\ast\ast$ \(p<0.01\), $\ast\ast\ast$ \(p<0.001\). Regression results to test the real income effect for 19 European countries during the period 2003-2016. Labor productivity is measured as the share of gross-output volumes ($Q$) over the total number of hours worked. TFP is calculated as the residual from an OLS regression of gross-output volumes ($Q$) on a translog production function including capital volumes ($K$), total number of hours worked ($L$) and intermediate input volumes ($M$). All regressions include: GDP growth, government consolidated gross debt as \% of GDP; government interest payable as \% of GDP; net government lending/borrowing as \% of GDP; gross fixed capital formation as \% of GDP; period average exchange rate; corporate tax rate; and country ($c$) and year ($t$) fixed effects.
    \end{table}

\FloatBarrier
%\newpage

\subsection{Controlling for changes in corporate taxation using Eurostat data}
\label{SM:robustness_ETR_Eurostat}
\FloatBarrier
\subsubsection{Taxation and automation}

    \begin{table}[H]
    \caption{Taxation and automation}
    { \centering
    \begin{adjustbox}{width=0.9\textwidth}
    \centering
    \begin{tabular}{l|cccc|cccc|ccc}
    \toprule \addlinespace
\csname @@input\endcsname{inputs/robustness/ETR_Eurostat/Results2shortV1_RICTint_ct_All_95t16}
\midrule
\csname @@input\endcsname{inputs/robustness/ETR_Eurostat/Results2shortV1_RICTint_ct_All_95t07}
\midrule
\csname @@input\endcsname{inputs/robustness/ETR_Eurostat/Results2shortV1_RICTint_ct_All_08t16}
\bottomrule
    \end{tabular}\end{adjustbox} \\ }
    \label{tab:regr_pre_tax_robots_ETR} \scriptsize
      Notes: $\ast$ \(p<0.05\), $\ast\ast$ \(p<0.01\), $\ast\ast\ast$ \(p<0.001\). Regression results of aggregate flows of tax revenues on different automation measures for 19 European countries during the period 2006-2016. All regressions use country level data and include: GDP growth, gross output share of the service sector in total economy; Herfindahl-Hirschman Index computed based on the gross-output shares of macro-sectors; government consolidated gross debt as \% of GDP; government interest payable as \% of GDP; net government lending/borrowing as \% of GDP; gross fixed capital formation as \% of GDP; period average exchange rate; effective tax rate; and country ($c$) and year ($t$) fixed effects. All regressions in Panel A also include the ln of gross-output value ($pQ$).
    \end{table}

\FloatBarrier
%\newpage

\subsubsection{Taxation and economic production}

	\begin{table}[!ht]
	{\centering 
    \caption{Taxation and the structure of economic production for the period 2006-2016}
    \begin{adjustbox}{width=\textwidth}\begin{tabular}{l|cccc|cccc|ccc}
    
    \toprule \addlinespace
\csname @@input\endcsname{inputs/robustness/ETR_Eurostat/Results2RICTint_ct_All_95t16}
\bottomrule
    \end{tabular}\end{adjustbox} \\ }

        \scriptsize
   Notes: $\ast$ \(p<0.05\), $\ast\ast$ \(p<0.01\), $\ast\ast\ast$ \(p<0.001\). Regression results to establish the link between tax aggregation and economic production for 19 European countries during the period 2006-2016. All regressions use country level data and include: GDP growth ($GDPgrowth_{c,t}$), share of gross output produced in service industries ($Services_{c,t}$); the Herfindahl-Hirschman Index computed based on the gross-output shares of macro-sectors ($HHI_{c,t}$); government consolidated gross debt as \% of GDP ($Debt^{\%GDP}_{c,t}$); government interest payable as \% of GDP ($Interest^{\%GDP}_{c,t}$); net government lending/borrowing as \% of GDP ($Lending^{\%GDP}_{c,t}$); gross fixed capital formation as \% of GDP ($GovInv^{\%GDP}_{c,t}$); period average exchange rate ($XRate_{c,t}$); effective tax rate ($ETR_{c,t}$); and country ($c$) and year ($t$) fixed effects. For the first block, $wL_{c,t}$, $rK_{c,t}$ and $pQ_{c,t}$ are expressed as the natural logarithm ($ln$) while for the last two blocks they are expressed as \% of GDP.
    \end{table}

	\begin{table}[!ht]
	{\centering 
     
    \caption{Taxation and the structure of economic production  for the period 2006-2007}
    \begin{adjustbox}{width=\textwidth}\begin{tabular}{l|cccc|cccc|ccc}
    
    \toprule \addlinespace

\csname @@input\endcsname{inputs/robustness/ETR_Eurostat/Results2RICTint_ct_All_95t07}
\bottomrule
    \end{tabular}\end{adjustbox} \\ }

        \scriptsize
   Notes: $\ast$ \(p<0.05\), $\ast\ast$ \(p<0.01\), $\ast\ast\ast$ \(p<0.001\). Regression results to establish the link between tax aggregation and economic production for 19 European countries during the period 2006-2007. All regressions use country level data and include: GDP growth ($GDPgrowth_{c,t}$), share of gross output produced in service industries ($Services_{c,t}$); the Herfindahl-Hirschman Index computed based on the gross-output shares of macro-sectors ($HHI_{c,t}$); government consolidated gross debt as \% of GDP ($Debt^{\%GDP}_{c,t}$); government interest payable as \% of GDP ($Interest^{\%GDP}_{c,t}$); net government lending/borrowing as \% of GDP ($Lending^{\%GDP}_{c,t}$); gross fixed capital formation as \% of GDP ($GovInv^{\%GDP}_{c,t}$); period average exchange rate ($XRate_{c,t}$); effective tax rate ($ETR_{c,t}$); and country ($c$) and year ($t$) fixed effects. For the first block, $wL_{c,t}$, $rK_{c,t}$ and $pQ_{c,t}$ are expressed as the natural logarithm ($ln$) while for the last two blocks they are expressed as \% of GDP.
    \end{table}

	\begin{table}[!ht]
	{\centering 
     
    \caption{Taxation and the structure of economic production after 2008}
    \begin{adjustbox}{width=\textwidth}\begin{tabular}{l|cccc|cccc|ccc}
    
    \toprule \addlinespace
\csname @@input\endcsname{inputs/robustness/ETR_Eurostat/Results2RICTint_ct_All_08t16}
\bottomrule
    \end{tabular}\end{adjustbox} \\ }

        \scriptsize
   Notes: $\ast$ \(p<0.05\), $\ast\ast$ \(p<0.01\), $\ast\ast\ast$ \(p<0.001\). Regression results to establish the link between tax aggregation and economic production for 19 European countries during the period 2008-2016. All regressions use country level data and include: GDP growth ($GDPgrowth_{c,t}$), share of gross output produced in service industries ($Services_{c,t}$); the Herfindahl-Hirschman Index computed based on the gross-output shares of macro-sectors ($HHI_{c,t}$); government consolidated gross debt as \% of GDP ($Debt^{\%GDP}_{c,t}$); government interest payable as \% of GDP ($Interest^{\%GDP}_{c,t}$); net government lending/borrowing as \% of GDP ($Lending^{\%GDP}_{c,t}$); gross fixed capital formation as \% of GDP ($GovInv^{\%GDP}_{c,t}$); period average exchange rate ($XRate_{c,t}$); effective tax rate ($ETR_{c,t}$); and country ($c$) and year ($t$) fixed effects. For the first block, $wL_{c,t}$, $rK_{c,t}$ and $pQ_{c,t}$ are expressed as the natural logarithm ($ln$) while for the last two blocks they are expressed as \% of GDP.
    \end{table}

\FloatBarrier	
\newpage
\subsubsection{The reinstatement effect}

		\begin{table}[!h]
    {\centering 
    \caption{The reinstatement effect}
    \label{tab:regr_reinstatement_ETR_Eurostat}
    \begin{adjustbox}{width=0.8\textwidth}\begin{tabular}{l|cccccc}
    
    \toprule \addlinespace

\csname @@input\endcsname{inputs/robustness/ETR_Eurostat/Results4shortRICTint_ct_All_95t16}
\bottomrule \addlinespace
\csname @@input\endcsname{inputs/robustness/ETR_Eurostat/Results4shortRICTint_ct_All_95t07}
\bottomrule \addlinespace
\csname @@input\endcsname{inputs/robustness/ETR_Eurostat/Results4shortRICTint_ct_All_08t16}
\bottomrule
    \end{tabular}\end{adjustbox}\\ }
    \scriptsize
    Notes: $\ast$ \(p<0.05\), $\ast\ast$ \(p<0.01\), $\ast\ast\ast$ \(p<0.001\). Regression results to test the reinstatement effect for 19 European countries during the period 2006-2016. All regressions include: GDP growth, government consolidated gross debt as \% of GDP; government interest payable as \% of GDP; net government lending/borrowing as \% of GDP; gross fixed capital formation as \% of GDP; period average exchange rate; value added TFP--calculated as the residual from an OLS regression of value-added volumes ($VA$) on a translog production function including capital volumes ($K$) and total number of hours worked ($L$); effective tax rate; and country ($c$) and year ($t$) fixed effects.
    \end{table}

\FloatBarrier
\newpage
\subsubsection{The real-income effect}

	\begin{table}[!h]
    {\centering 
        \caption{The real income effect}
            \label{tab:regr_realincome_ETR_Eurostat}

    \begin{adjustbox}{width=\textwidth}\begin{tabular}{l|cccccccc}
    \toprule \addlinespace
\csname @@input\endcsname{inputs/robustness/ETR_Eurostat/Results5RICTint_ct_All_95t16}
\bottomrule \addlinespace
\csname @@input\endcsname{inputs/robustness/ETR_Eurostat/Results5RICTint_ct_All_95t07}
\bottomrule \addlinespace
\csname @@input\endcsname{inputs/robustness/ETR_Eurostat/Results5RICTint_ct_All_08t16}
\bottomrule
    \end{tabular}\end{adjustbox}\\ \noindent }
    \scriptsize
    Notes: $\ast$ \(p<0.05\), $\ast\ast$ \(p<0.01\), $\ast\ast\ast$ \(p<0.001\). Regression results to test the real income effect for 19 European countries during the period 2006-2016. Labor productivity is measured as the share of gross-output volumes ($Q$) over the total number of hours worked. TFP is calculated as the residual from an OLS regression of gross-output volumes ($Q$) on a translog production function including capital volumes ($K$), total number of hours worked ($L$) and intermediate input volumes ($M$). All regressions include: GDP growth, government consolidated gross debt as \% of GDP; government interest payable as \% of GDP; net government lending/borrowing as \% of GDP; gross fixed capital formation as \% of GDP; period average exchange rate; effective tax rate; and country ($c$) and year ($t$) fixed effects.
    \end{table}

\FloatBarrier
%\newpage

\subsection{Controlling for trade}
\label{SM:robustness_trade}
\FloatBarrier
\subsubsection{Taxation and automation}

    \begin{table}[H]
    \caption{Taxation and automation}
    { \centering
    \begin{adjustbox}{width=0.85\textwidth}
    \centering
    \begin{tabular}{l|cccc|cccc|ccc}
    \toprule \addlinespace
\csname @@input\endcsname{inputs/robustness/Trade_OECD/Results2shortV1_RICTint_ct_All_95t16}
\midrule
\csname @@input\endcsname{inputs/robustness/Trade_OECD/Results2shortV1_RICTint_ct_All_95t07}
\midrule
\csname @@input\endcsname{inputs/robustness/Trade_OECD/Results2shortV1_RICTint_ct_All_08t16}
\bottomrule
    \end{tabular}\end{adjustbox} \\ }
    \label{tab:regr_pre_tax_robots_Trade} \scriptsize
  Notes: $\ast$ \(p<0.05\), $\ast\ast$ \(p<0.01\), $\ast\ast\ast$ \(p<0.001\). Regression results of aggregate flows of tax revenues on different automation measures for 19 European countries during the period 1995-2016. All regressions use country level data and include: GDP growth, gross output share of the service sector in total economy; Herfindahl-Hirschman Index computed based on the gross-output shares of macro-sectors; government consolidated gross debt as \% of GDP; government interest payable as \% of GDP; net government lending/borrowing as \% of GDP; gross fixed capital formation as \% of GDP; period average exchange rate; imports as \% of GDP; exports as \% of GDP; and country ($c$) and year ($t$) fixed effects. All regressions in Panel A also include the ln of gross-output value ($pQ$).
    \end{table}

\FloatBarrier
\newpage
\subsubsection{Taxation and economic production}

	\begin{table}[!ht]
	{\centering 
     
    \caption{Taxation and the structure of economic production}
    \begin{adjustbox}{width=\textwidth}\begin{tabular}{l|cccc|cccc|ccc}
    
    \toprule \addlinespace
\csname @@input\endcsname{inputs/robustness/Trade_OECD/Results2RICTint_ct_All_95t16}
\bottomrule
    \end{tabular}\end{adjustbox} \\ }

        \scriptsize
   Notes: $\ast$ \(p<0.05\), $\ast\ast$ \(p<0.01\), $\ast\ast\ast$ \(p<0.001\). Regression results to establish the link between tax aggregation and economic production for 19 European countries during the period 1995-2016. All regressions use country level data and include: GDP growth ($GDPgrowth_{c,t}$), share of gross output produced in service industries ($Services_{c,t}$); the Herfindahl-Hirschman Index computed based on the gross-output shares of macro-sectors ($HHI_{c,t}$); government consolidated gross debt as \% of GDP ($Debt^{\%GDP}_{c,t}$); government interest payable as \% of GDP ($Interest^{\%GDP}_{c,t}$); net government lending/borrowing as \% of GDP ($Lending^{\%GDP}_{c,t}$); gross fixed capital formation as \% of GDP ($GovInv^{\%GDP}_{c,t}$); period average exchange rate ($XRate_{c,t}$); imports as \% of GDP ($Imports^{\%GDP}_{c,t}$); exports as \% of GDP ($Exports^{\%GDP}_{c,t}$); and country ($c$) and year ($t$) fixed effects. For the first block, $wL_{c,t}$, $rK_{c,t}$ and $pQ_{c,t}$ are expressed as the natural logarithm ($ln$) while for the last two blocks they are expressed as \% of GDP.
    \end{table}

	\begin{table}[!ht]
	{\centering 
     
    \caption{Taxation and the structure of economic production before 2007}
    \begin{adjustbox}{width=\textwidth}\begin{tabular}{l|cccc|cccc|ccc}
    
    \toprule \addlinespace

\csname @@input\endcsname{inputs/robustness/Trade_OECD/Results2RICTint_ct_All_95t07}
\bottomrule
    \end{tabular}\end{adjustbox} \\ }

        \scriptsize
   Notes: $\ast$ \(p<0.05\), $\ast\ast$ \(p<0.01\), $\ast\ast\ast$ \(p<0.001\). Regression results to establish the link between tax aggregation and economic production for 19 European countries during the period 1995-2007. All regressions use country level data and include: GDP growth ($GDPgrowth_{c,t}$), share of gross output produced in service industries ($Services_{c,t}$); the Herfindahl-Hirschman Index computed based on the gross-output shares of macro-sectors ($HHI_{c,t}$); government consolidated gross debt as \% of GDP ($Debt^{\%GDP}_{c,t}$); government interest payable as \% of GDP ($Interest^{\%GDP}_{c,t}$); net government lending/borrowing as \% of GDP ($Lending^{\%GDP}_{c,t}$); gross fixed capital formation as \% of GDP ($GovInv^{\%GDP}_{c,t}$); period average exchange rate ($XRate_{c,t}$); imports as \% of GDP ($Imports^{\%GDP}_{c,t}$); exports as \% of GDP ($Exports^{\%GDP}_{c,t}$); and country ($c$) and year ($t$) fixed effects. For the first block, $wL_{c,t}$, $rK_{c,t}$ and $pQ_{c,t}$ are expressed as the natural logarithm ($ln$) while for the last two blocks they are expressed as \% of GDP.
    \end{table}

	\begin{table}[!ht]
	{\centering 
     
    \caption{Taxation and the structure of economic production after 2008}
    \begin{adjustbox}{width=\textwidth}\begin{tabular}{l|cccc|cccc|ccc}
    
    \toprule \addlinespace
\csname @@input\endcsname{inputs/robustness/Trade_OECD/Results2RICTint_ct_All_08t16}
\bottomrule
    \end{tabular}\end{adjustbox} \\ }

        \scriptsize
   Notes: $\ast$ \(p<0.05\), $\ast\ast$ \(p<0.01\), $\ast\ast\ast$ \(p<0.001\). Regression results to establish the link between tax aggregation and economic production for 19 European countries during the period 2008-2016. All regressions use country level data and include: GDP growth ($GDPgrowth_{c,t}$), share of gross output produced in service industries ($Services_{c,t}$); the Herfindahl-Hirschman Index computed based on the gross-output shares of macro-sectors ($HHI_{c,t}$); government consolidated gross debt as \% of GDP ($Debt^{\%GDP}_{c,t}$); government interest payable as \% of GDP ($Interest^{\%GDP}_{c,t}$); net government lending/borrowing as \% of GDP ($Lending^{\%GDP}_{c,t}$); gross fixed capital formation as \% of GDP ($GovInv^{\%GDP}_{c,t}$); period average exchange rate ($XRate_{c,t}$); imports as \% of GDP ($Imports^{\%GDP}_{c,t}$); exports as \% of GDP ($Exports^{\%GDP}_{c,t}$); and country ($c$) and year ($t$) fixed effects. For the first block, $wL_{c,t}$, $rK_{c,t}$ and $pQ_{c,t}$ are expressed as the natural logarithm ($ln$) while for the last two blocks they are expressed as \% of GDP.
    \end{table}

\FloatBarrier	
\newpage
\subsubsection{The reinstatement effect}

		\begin{table}[!h]
    {\centering 
    \caption{The reinstatement effect}
    \label{tab:regr_reinstatement_trade}
    \begin{adjustbox}{width=0.8\textwidth}\begin{tabular}{l|cccccc}
    
    \toprule \addlinespace

\csname @@input\endcsname{inputs/robustness/Trade_OECD/Results4shortRICTint_ct_All_95t16}
\bottomrule \addlinespace
\csname @@input\endcsname{inputs/robustness/Trade_OECD/Results4shortRICTint_ct_All_95t07}
\bottomrule \addlinespace
\csname @@input\endcsname{inputs/robustness/Trade_OECD/Results4shortRICTint_ct_All_08t16}
\bottomrule
    \end{tabular}\end{adjustbox}\\ }
    \scriptsize
    Notes: $\ast$ \(p<0.05\), $\ast\ast$ \(p<0.01\), $\ast\ast\ast$ \(p<0.001\). Regression results to test the reinstatement effect for 19 European countries during the period 1995-2016. All regressions include: GDP growth, government consolidated gross debt as \% of GDP; government interest payable as \% of GDP; net government lending/borrowing as \% of GDP; gross fixed capital formation as \% of GDP; period average exchange rate; value added TFP--calculated as the residual from an OLS regression of value-added volumes ($VA$) on a translog production function including capital volumes ($K$) and total number of hours worked ($L$); imports as \% of GDP; exports as \% of GDP; and country ($c$) and year ($t$) fixed effects.
    \end{table}

\FloatBarrier
\newpage
\subsubsection{The real-income effect}

	\begin{table}[!h]
    {\centering 
        \caption{The real income effect}
            \label{tab:regr_realincome_trade}

    \begin{adjustbox}{width=\textwidth}\begin{tabular}{l|cccccccc}
    \toprule \addlinespace
\csname @@input\endcsname{inputs/robustness/Trade_OECD/Results5RICTint_ct_All_95t16}
\bottomrule \addlinespace
\csname @@input\endcsname{inputs/robustness/Trade_OECD/Results5RICTint_ct_All_95t07}
\bottomrule \addlinespace
\csname @@input\endcsname{inputs/robustness/Trade_OECD/Results5RICTint_ct_All_08t16}
\bottomrule
    \end{tabular}\end{adjustbox}\\ \noindent }
    \scriptsize
    Notes: $\ast$ \(p<0.05\), $\ast\ast$ \(p<0.01\), $\ast\ast\ast$ \(p<0.001\). Regression results to test the real income effect for 19 European countries during the period 1995-2016. Labor productivity is measured as the share of gross-output volumes ($Q$) over the total number of hours worked. TFP is calculated as the residual from an OLS regression of gross-output volumes ($Q$) on a translog production function including capital volumes ($K$), total number of hours worked ($L$) and intermediate input volumes ($M$). All regressions include: GDP growth, government consolidated gross debt as \% of GDP; government interest payable as \% of GDP; net government lending/borrowing as \% of GDP; gross fixed capital formation as \% of GDP; period average exchange rate; imports as \% of GDP; exports as \% of GDP; and country ($c$) and year ($t$) fixed effects.
    \end{table}

\FloatBarrier
\newpage
\subsection{The progressiveness of taxation}
\label{SM:robustness_progressive}

%\subsubsection{Whole Europe}
	\begin{table}[!ht]
	{\centering 
     
    \caption{Taxation and the structure of economic production}
    \begin{adjustbox}{width=\textwidth}
    \begin{tabular}{l|cccc|cccc|ccc}
    
    \toprule \addlinespace
\csname @@input\endcsname{inputs/robustness/TaxProgressiveness/Results2RICTint_ct_All_95t16}
\bottomrule
    \end{tabular}\end{adjustbox} \\ }

        \scriptsize
   Notes: $\ast$ \(p<0.05\), $\ast\ast$ \(p<0.01\), $\ast\ast\ast$ \(p<0.001\). Regression results to establish the link between tax aggregation and economic production for 19 European countries during the period 1995-2016. All regressions use country level data and include: GDP growth ($GDPgrowth_{c,t}$), share of gross output produced in service industries ($Services_{c,t}$); the Herfindahl-Hirschman Index computed based on the gross-output shares of macro-sectors ($HHI_{c,t}$); government consolidated gross debt as \% of GDP ($Debt^{\%GDP}_{c,t}$); government interest payable as \% of GDP ($Interest^{\%GDP}_{c,t}$); net government lending/borrowing as \% of GDP ($Lending^{\%GDP}_{c,t}$); gross fixed capital formation as \% of GDP ($GovInv^{\%GDP}_{c,t}$); period average exchange rate ($XRate_{c,t}$); Gini index from the industry level distribution of hourly wage ($Gini^{w}_{c,t}$); and country ($c$) and year ($t$) fixed effects. For the first block, $wL_{c,t}$, $rK_{c,t}$ and $pQ_{c,t}$ are expressed as the natural logarithm ($ln$) while for the last two blocks they are expressed as \% of GDP.
    \end{table}

	\begin{table}[!ht]
	{\centering 
     
    \caption{Taxation and the structure of economic production before 2007}
    \begin{adjustbox}{width=\textwidth}\begin{tabular}{l|cccc|cccc|ccc}
    
    \toprule \addlinespace

\csname @@input\endcsname{inputs/robustness/TaxProgressiveness/Results2RICTint_ct_All_95t07}
\bottomrule
    \end{tabular}\end{adjustbox} \\ }

        \scriptsize
   Notes: $\ast$ \(p<0.05\), $\ast\ast$ \(p<0.01\), $\ast\ast\ast$ \(p<0.001\). Regression results to establish the link between tax aggregation and economic production for 19 European countries during the period 1995-2007. All regressions use country level data and include: GDP growth ($GDPgrowth_{c,t}$), share of gross output produced in service industries ($Services_{c,t}$); the Herfindahl-Hirschman Index computed based on the gross-output shares of macro-sectors ($HHI_{c,t}$); government consolidated gross debt as \% of GDP ($Debt^{\%GDP}_{c,t}$); government interest payable as \% of GDP ($Interest^{\%GDP}_{c,t}$); net government lending/borrowing as \% of GDP ($Lending^{\%GDP}_{c,t}$); gross fixed capital formation as \% of GDP ($GovInv^{\%GDP}_{c,t}$); period average exchange rate ($XRate_{c,t}$); Gini index from the industry level distribution of hourly wage ($Gini^{w}_{c,t}$); and country ($c$) and year ($t$) fixed effects. For the first block, $wL_{c,t}$, $rK_{c,t}$ and $pQ_{c,t}$ are expressed as the natural logarithm ($ln$) while for the last two blocks they are expressed as \% of GDP.
    \end{table}

	\begin{table}[!ht]
	{\centering 
     
    \caption{Taxation and the structure of economic production after 2008}
    \begin{adjustbox}{width=\textwidth}\begin{tabular}{l|cccc|cccc|ccc}
    
    \toprule \addlinespace
\csname @@input\endcsname{inputs/robustness/TaxProgressiveness/Results2RICTint_ct_All_08t16}
\bottomrule
    \end{tabular}\end{adjustbox} \\ }

        \scriptsize
   Notes: $\ast$ \(p<0.05\), $\ast\ast$ \(p<0.01\), $\ast\ast\ast$ \(p<0.001\). Regression results to establish the link between tax aggregation and economic production for 19 European countries during the period 2008-2016. All regressions use country level data and include: GDP growth ($GDPgrowth_{c,t}$), share of gross output produced in service industries ($Services_{c,t}$); the Herfindahl-Hirschman Index computed based on the gross-output shares of macro-sectors ($HHI_{c,t}$); government consolidated gross debt as \% of GDP ($Debt^{\%GDP}_{c,t}$); government interest payable as \% of GDP ($Interest^{\%GDP}_{c,t}$); net government lending/borrowing as \% of GDP ($Lending^{\%GDP}_{c,t}$); gross fixed capital formation as \% of GDP ($GovInv^{\%GDP}_{c,t}$); period average exchange rate ($XRate_{c,t}$); Gini index from the industry level distribution of hourly wage ($Gini^{w}_{c,t}$); and country ($c$) and year ($t$) fixed effects. For the first block, $wL_{c,t}$, $rK_{c,t}$ and $pQ_{c,t}$ are expressed as the natural logarithm ($ln$) while for the last two blocks they are expressed as \% of GDP.
    \end{table}

\FloatBarrier
\newpage

\subsection{Excluding OECD group 1100 ``taxes on income, profits and capital gains of individuals'' from capital taxes}
\label{SM:robustness_Tk}
\FloatBarrier
\subsubsection{Taxation and automation}

    \begin{table}[H]
    \caption{Taxation and automation}
    { \centering
    \begin{adjustbox}{width=0.85\textwidth}
    \centering
    \begin{tabular}{l|cccc|cccc|ccc}
    \toprule \addlinespace
\csname @@input\endcsname{inputs/robustness/Tk_alt/Results2shortV1_RICTint_ct_All_95t16}
\midrule
\csname @@input\endcsname{inputs/robustness/Tk_alt/Results2shortV1_RICTint_ct_All_95t07}
\midrule
\csname @@input\endcsname{inputs/robustness/Tk_alt/Results2shortV1_RICTint_ct_All_08t16}
\bottomrule
    \end{tabular}\end{adjustbox} \\ }
    \label{tab:regr_pre_tax_robots_Trade} \scriptsize
  Notes: $\ast$ \(p<0.05\), $\ast\ast$ \(p<0.01\), $\ast\ast\ast$ \(p<0.001\). Regression results of aggregate flows of tax revenues on different automation measures for 19 European countries during the period 1995-2016. All regressions use country level data and include: GDP growth, gross output share of the service sector in total economy; Herfindahl-Hirschman Index computed based on the gross-output shares of macro-sectors; government consolidated gross debt as \% of GDP; government interest payable as \% of GDP; net government lending/borrowing as \% of GDP; gross fixed capital formation as \% of GDP; period average exchange rate; and country ($c$) and year ($t$) fixed effects. All regressions in Panel A also include the ln of gross-output value ($pQ$). Taxes on capital $T^k$ exclude the OECD tax category 1100 ``taxes on income, profits and capital gains of individuals''.
    \end{table}

	\begin{table}[!ht]
	{\centering 
     
    \caption{Taxation and the structure of economic production before 2007}
    \begin{adjustbox}{width=\textwidth}\begin{tabular}{l|cccc|cccc|ccc}
    
    \toprule \addlinespace

\csname @@input\endcsname{inputs/robustness/Tk_alt/Results2RICTint_ct_All_95t07}
\bottomrule
    \end{tabular}\end{adjustbox} \\ }

        \scriptsize
   Notes: $\ast$ \(p<0.05\), $\ast\ast$ \(p<0.01\), $\ast\ast\ast$ \(p<0.001\). Regression results to establish the link between tax aggregation and economic production for 19 European countries during the period 1995-2007. All regressions use country level data and include: GDP growth ($GDPgrowth_{c,t}$), share of gross output produced in service industries ($Services_{c,t}$); the Herfindahl-Hirschman Index computed based on the gross-output shares of macro-sectors ($HHI_{c,t}$); government consolidated gross debt as \% of GDP ($Debt^{\%GDP}_{c,t}$); government interest payable as \% of GDP ($Interest^{\%GDP}_{c,t}$); net government lending/borrowing as \% of GDP ($Lending^{\%GDP}_{c,t}$); gross fixed capital formation as \% of GDP ($GovInv^{\%GDP}_{c,t}$); period average exchange rate ($XRate_{c,t}$);  and country ($c$) and year ($t$) fixed effects. For the first block, $wL_{c,t}$, $rK_{c,t}$ and $pQ_{c,t}$ are expressed as the natural logarithm ($ln$) while for the last two blocks they are expressed as \% of GDP. Taxes on capital $T^k$ exclude the OECD tax category 1100 ``taxes on income, profits and capital gains of individuals''.
    \end{table}

	\begin{table}[!ht]
	{\centering 
     
    \caption{Taxation and the structure of economic production after 2008}
    \begin{adjustbox}{width=\textwidth}\begin{tabular}{l|cccc|cccc|ccc}
    
    \toprule \addlinespace
\csname @@input\endcsname{inputs/robustness/Tk_alt/Results2RICTint_ct_All_08t16}
\bottomrule
    \end{tabular}\end{adjustbox} \\ }

        \scriptsize
   Notes: $\ast$ \(p<0.05\), $\ast\ast$ \(p<0.01\), $\ast\ast\ast$ \(p<0.001\). Regression results to establish the link between tax aggregation and economic production for 19 European countries during the period 2008-2016. All regressions use country level data and include: GDP growth ($GDPgrowth_{c,t}$), share of gross output produced in service industries ($Services_{c,t}$); the Herfindahl-Hirschman Index computed based on the gross-output shares of macro-sectors ($HHI_{c,t}$); government consolidated gross debt as \% of GDP ($Debt^{\%GDP}_{c,t}$); government interest payable as \% of GDP ($Interest^{\%GDP}_{c,t}$); net government lending/borrowing as \% of GDP ($Lending^{\%GDP}_{c,t}$); gross fixed capital formation as \% of GDP ($GovInv^{\%GDP}_{c,t}$); period average exchange rate ($XRate_{c,t}$); and country ($c$) and year ($t$) fixed effects. For the first block, $wL_{c,t}$, $rK_{c,t}$ and $pQ_{c,t}$ are expressed as the natural logarithm ($ln$) while for the last two blocks they are expressed as \% of GDP. Taxes on capital $T^k$ exclude the OECD tax category 1100 ``taxes on income, profits and capital gains of individuals''.
    \end{table}

\FloatBarrier
\newpage
